# Supplementary material for: MADOD: Generalizing OOD Detection to Unseen Domains via G-Invariance Meta-Learning
Source: arXiv:2411.02444 source file (2024-11-02)
Supplement: Supplementary file 1 [file x_appendix.tex]

\subsection{Notations}
For clear interpretation, we list the notations used in this paper, along with their corresponding explanations. This list is presented in Table~\ref{tab:notations} for easy reference.

\begin{table}[!ht]
    \centering
    \small
    \caption{Important notations and corresponding descriptions.}
    % \begin{tabular}{c|p{2.4in}}
    \begin{tabular}{c|c}
       \toprule
        \textbf{Notations} & \textbf{Descriptions} \\
        \midrule
        $e, e^{'}$ & a domain, a synthetic domain \\
        $\mathcal{E}_{\text{\text{all}}}, \mathcal{E}_{\text{train}}$ & set of all domains, set of training domains\\
        $\mathbf{x},y$ &  data instance and its label\\
        $\mathbf{x}^e$ &  data instance of domain e \\
        $\mathcal{X}, \mathcal{Y}$ & input space, output space \\
        $(X,Y)$ & pair of random variables for inputs and labels \\
        $(X^e, Y^e)$ & pair of random variables associated with domain e \\
        $\mathbb{P}_{\text{ID}}(\cdot), \mathbb{P}_{\text{OOD}}(\cdot)$ & ID data distribution and OOD data distribution \\
        $\mathbb{P}_{\text{ID}}(X, Y)$ & ID data distribution \\
        $\mathbb{P}_{\text{ID}}(X^e, Y^e)$ & ID joint distribution associated with domain $e$ \\
        $\mathcal{D}, \mathcal{D}^e, \mathcal{D}_{\text{AugOOD}}$  & the entire dataset, subset of data that belongs to the domain $e$, augmented OODs \\
        % $\mathcal{D}, \mathcal{D}_{te}$ & training and testing datasets\\
        % $E_{tr}, E_{te}$ & numbers of training and testing domains\\
        % $\mathcal{D}^e, |\mathcal{D}^e|$ & data of domain $e$, size of data of domain $e$  \\
        % $\mathcal{Y}_{tr}, \mathcal{Y}_{te}$ & label spaces of training and testing datasets \\
        $K$ & total number of training classes \\
        % $y_{ID}, y_{OOD}$ & labels of testing data \\
        $\mathbf{f}$ & the predictor \\
        $\ell$ & the loss function\\
        $\mathbf{g},\mathbf{h}$ & featurizer and classifier of the predictor $f$\\
        $\bm{\theta}, \bm{\phi}, \bm{\psi}$ & parameters of $f$, $g$, and $h$, respectively \\
        $\hat{\bm{\theta}}, \hat{\bm{\phi}}, \hat{\bm{\psi}}$ & the optimal parameters of $f$, $g$, and $h$ that satisfy $G$-invariance \\
        $\Phi$ & all possible configurations of $\hat{\bm{\phi}}$ \\
        $o(\cdot)$ & OOD detector \\
        $q_\omega(\cdot)$ & the DDU OOD detector with density threshold $\omega$ \\
        $\boldsymbol{\theta}, \boldsymbol{\theta}_g, \boldsymbol{\theta}_h$ & parameters of the predictor, the featurizer, and the classifier \\
        % $\Theta$ & parameter space\\
        $G$ & the transformation model\\
        $E_s, E_v, D$ & semantic encoder, the variation encoder, and the decoder\\
        $\mathcal{S, V}$ & latent semantic and variation spaces\\
        $\mathbf{s}, \mathbf{v}$ & semantic and variation factors\\
        $R_{\text{SGI}}$ & the semantic $G$-invariance regularization term\\
        $d$ & distance metrics\\
        $R_{\text{OOD}}$ & the OOD regularization term\\
        $\lambda_1,\lambda_2$ & mixing coefficients\\
        $\hat{\mathbf{s}}$ & semantic factor generated using the mixup\\
        $\hat{\mathbf{x}}$ & augmented pseudo-OOD instance\\
        % $\mathcal{D}_{pseudo}$ & dataset of pseudo-OODs\\
        $\xi$ & empirical threshold qualifying pseudo-OODs\\
        $\mathbf{x}_{I},\mathbf{x}_{O}$ & ID instance, OOD instance\\
        % $\mathbf{x}_{out},y_{OOD}$ & pseudo-OOD instances\\
        $m_{I}, m_{O}$ & ID and OOD energy margins\\
        $E_g$ & energy function\\
        $T$ & temperature parameter\\
        $\beta_1,\beta_2$ & Lagrangian multipliers (dual variables)\\
        $\gamma_1,\gamma_2$ & error tolerance margins of the $R_{\text{SGI}}$ and $R_{\text{OOD}}$, respectively\\
        $\eta_p,\eta_{sgi},\eta_{ood}$ & learning rates of primal and dual parameters\\
       \bottomrule
    \end{tabular}
    \label{tab:notations}
\end{table}

\subsection{Algorithm of \sysname{}}
Following are the pseudo-codes for the \sysname{}:

\begin{algorithm}[t]
    \caption{\sysname{}}
    \label{alg:our_alg}
    \begin{flushleft}
        \textbf{Require}: A pre-trained model $G=\{E_s,E_v, D\}$, fitted GDA using $\{(E_s(\mathbf{x}_i),y_i)\}_{i=1}^{|\mathcal{D}|}$, and the energy score function $E_g$.\\
        \textbf{Require}: Mixing parameters $\lambda_1,\lambda_2$, the threshold of GDA $\xi$, energy scoring margins $m_{I},m_{O}$, the temperature parameter $T$, regularization margins $\gamma_1,\gamma_2$, primal and dual learning rate $\eta_p,\eta_{dg},\eta_{ood}$.
    \end{flushleft}
\begin{algorithmic}[1]
    
    \Repeat
        \For{minibatch $\{(\mathbf{x}_i,y_i)\}_{i=1}^m$ in training data $\mathcal{D}$}
        \State $\mathcal{L}_{cls}\leftarrow(1/m)\sum_{i=1}^m\mathcal{L}_{CE}(f_{\boldsymbol{\theta}}(\mathbf{x}_i),y_i)$
        \State $(\Tilde{\mathbf{x}}_i,y_i)\leftarrow\textsc{DataAug}(\mathbf{x}_i,y_i),\: \forall i\in[m]$
        \State $R_{\text{SGI}}\leftarrow(1/m)\sum_{i=1}^m d[g_{\bm{\phi}}(\mathbf{x}_i), g_{\bm{\phi}}(\Tilde{\mathbf{x}}_i)]$
        \State $\mathcal{D}_{\text{AugOOD}}\leftarrow\emptyset$
        % \State Fitting GDA using $\{(E_s(\mathbf{x}_i),y_i)\}_{i=1}^m$
        \For{each $(\mathbf{x}_i,y_i)$ in the minibatch}
            \State \multiline{%
                Sample $(\mathbf{x}_j,y_j)$ from $\mathcal{D}$, $y_i\neq y_j$}
            \State $\hat{\mathbf{s}}=\lambda_1\cdot E_s(\mathbf{x}_i) + \lambda_2\cdot E_s(\mathbf{x}_j)$
            \If{GDA($\hat{\mathbf{s}})<\xi$}
                \State \multiline{%
                    Add $(D(\hat{\mathbf{s}},\mathbf{v}),0)$ to $\mathcal{D}_{\text{AugOOD}}$ where $\mathbf{v}\sim\mathcal{N}(0,\mathbf{I})$}
            \EndIf
        \EndFor
        \State $n\leftarrow|\mathcal{D}_{\text{AugOOD}}|$
        \State \multiline{%
            Evaluate $R_{\text{OOD}}$ using Equation~(\ref{eq:reg-ood})
            % $R_{\text{OOD}}\leftarrow(1/m)\sum_{i=1}^m(\max(0,E_g(\mathbf{x}_i,\boldsymbol{\theta})-m_{in}))^2+(1/n)\sum_{l=1}^n( \max(0,m_{out}-E_g(\mathbf{x}_l,\boldsymbol{\theta})) )^2$
        }
        \State $\ell(\boldsymbol{\theta})\leftarrow\mathcal{L}_{cls}+\beta_1\cdot R_{\text{SGI}} + \beta_2\cdot R_{\text{OOD}}$
        \State $\boldsymbol{\theta}\leftarrow\text{Adam}(\ell(\boldsymbol{\theta}),\boldsymbol{\theta},\eta_p)$
        \State $\beta_1\leftarrow\max\{0, \beta_1+\eta_{dg}\cdot(R_{\text{SGI}}-\gamma_1)\}$
        \State $\beta_2\leftarrow\max\{0, \beta_2+\eta_{ood}\cdot(R_{\text{OOD}}-\gamma_2)\}$
        \EndFor
    \Until{$\text{convergence}$}

    \Procedure{\textsc{DataAug}}{$\mathbf{x},y$}
        \State $\mathbf{s}\leftarrow E_s(\mathbf{x})$, $\mathbf{v}\leftarrow E_v(\mathbf{x})$
        \State Sample $\mathbf{v}'\sim\mathcal{N}(0,\mathbf{I})$
        \State \textbf{return } $(D(\mathbf{s},\mathbf{v}'),y)$
    \EndProcedure
\end{algorithmic}
\end{algorithm}

\subsection{\texorpdfstring{Architecture of the Transformation Model $G$ and the Predictor $f$}{Architecture of the Transformation Model G and the Predictor f}}
% All the images are resized to 224$\times$224. 
The semantic encoder $E_s$ is made of four convolution layers. The first one has 64 filters, and each of the others has 128 filters. The kernel sizes are (7,7), (4,4), (3,3), and (3,3) for layers 1-4, respectively. The stride of the second layer is (2,2), and the stride of all the other layers is (1,1). The activation function of the first three layers is ReLU. The last convolution layer does not have an activation function. The variation encoder $E_v$ is made of 6 convolution layers, and there is an adaptive average pooling layer with output size 1 between the last two convolution layers. The numbers of filters are 64, 128, 256, 256, 256, and 2 for the convolution layers, respectively. The kernel sizes are (7,7), (4,4), (4,4), (4,4), (4,4), (1,1). And the strides are (1,1), (2,2), (2,2), (2,2), (2,2), (1,1). The activation function of the first five layers is ReLU. The last convolution layer does not have an activation function. The decoder $D$ is made of 4 convolution layers followed by an average pooling layer whose kernel size is 3, stride is 2, and padding is [1,1]. The numbers of filters of the convolution layers are 64, 128, 256, 1, respectively. The kernel sizes are (4,4) for the first three convolution layers and (1,1) for the fourth convolution layer. The strides are (2,2) for the first three convolution layers and (1,1) for the fourth convolution layer. The first three convolution layers' activation functions are LeakyReLU. The other layers do not have activation functions. The training of $G$ is an end-to-end training.
As for the predictor $f$, $g$ is Resnet50 \cite{he2016deep}, and $h$ is a fully connected layer with input size 2048 and output size $K$.

% More transformed image examples are shown in Figure~\ref{fig:transformed-images}.

% \begin{figure*}[t]
%     \centering
%     \includegraphics[width=0.8\linewidth]{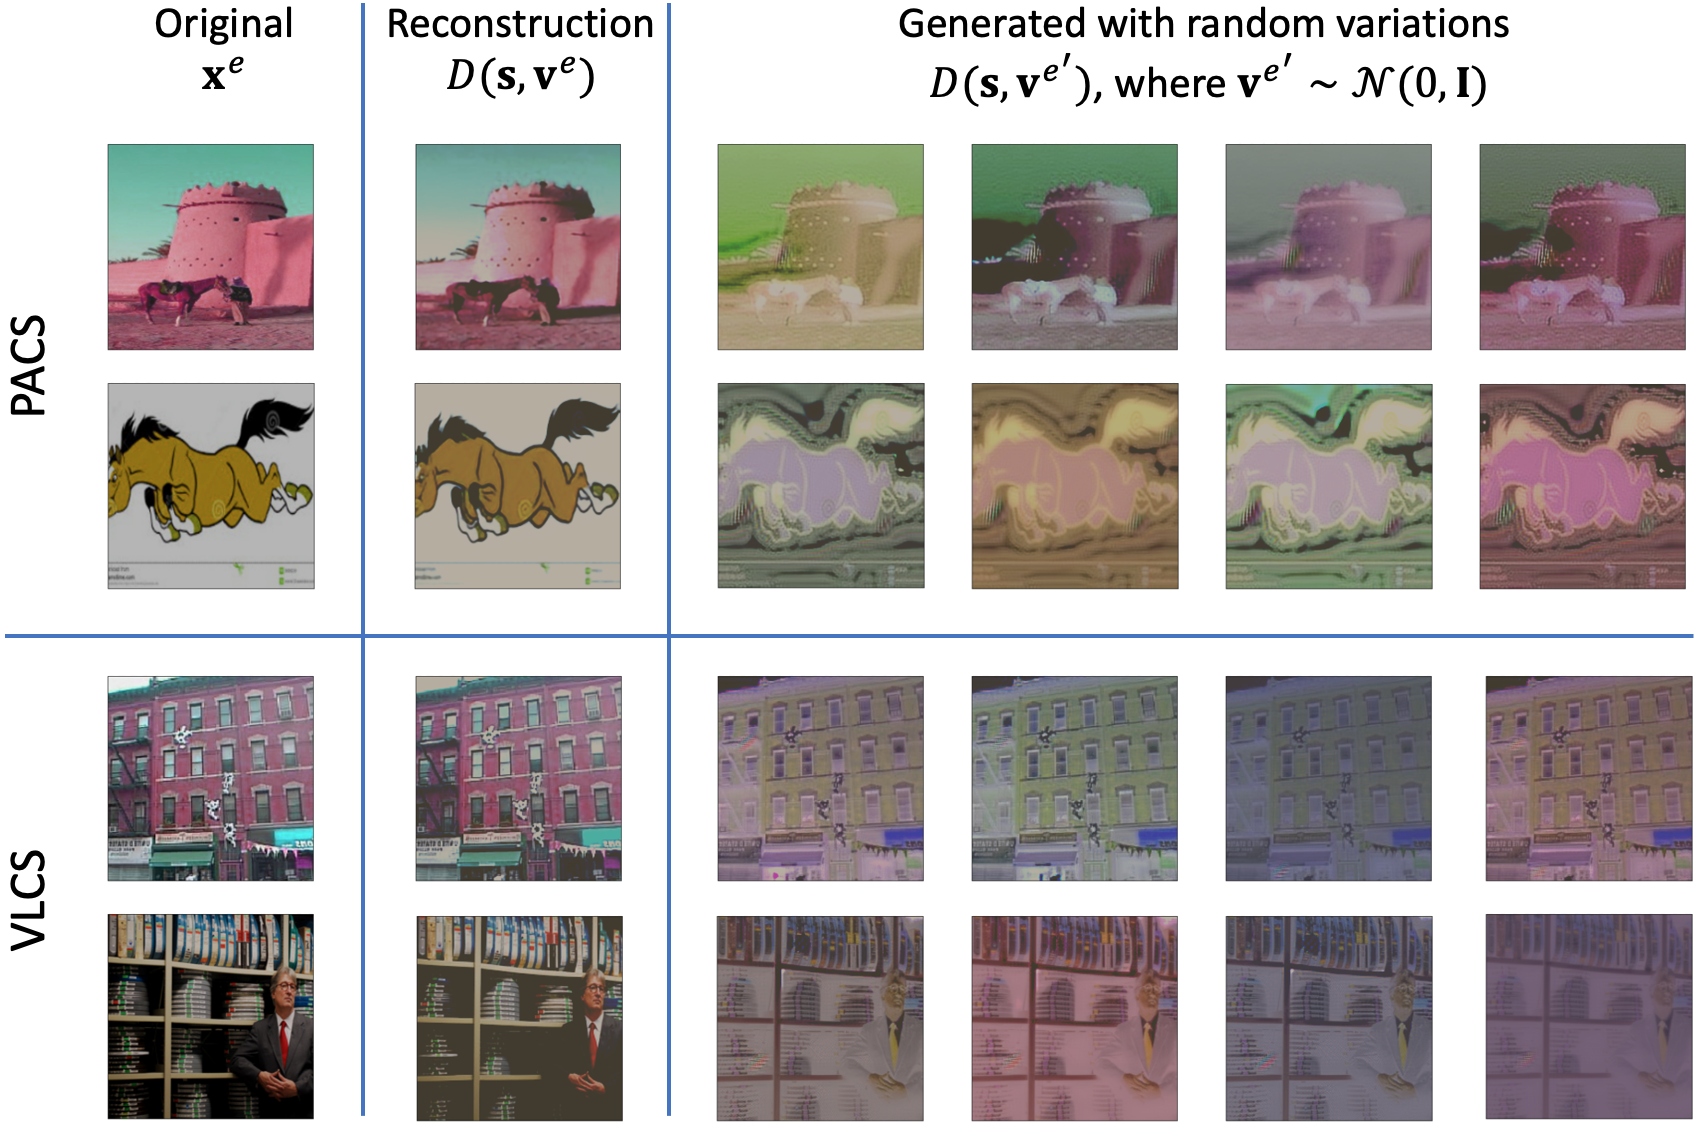}
%     \caption{More transformed image examples generated using $G$ with randomly sampled variation factors.
%     }
%     \label{fig:transformed-images}
% \end{figure*}

% \subsection{Training $G$}

\subsection{Proofs}
\label{appendix:proofs}
\begin{customthm}{1}
    semantic $G$-invariance implies $G$-invariance, but not vice versa. %\label{prop:Semantic-G-invariance}
\end{customthm}
\begin{proof}
We begin by defining the concept of $G$-invariance, where a predictor \( f \) is considered G-invariant if it satisfies the condition \( f(\mathbf{x}) = f(G(\mathbf{x}, e)) \) for any data instance \( \mathbf{x} \) and transformation \( e \). This definition implies that the output of \( f \) remains unchanged under the application of the transformation function \( G \).

semantic $G$-invariance (SGI), on the other hand, is a more specific form of invariance that focuses on the consistency of semantic representations across transformations. A predictor \( f = g \circ h \) is semantically G-invariant if the semantic representation \( g(\mathbf{x}) \) remains consistent for both the original data \( \mathbf{x} \) and its transformed version \( G(\mathbf{x}, e) \), i.e., \( g(\mathbf{x}) = g(G(\mathbf{x}, e)) \) for all \( \mathbf{x} \) and \( e \).

To prove that semantic $G$-invariance implies $G$-invariance, we assume that a predictor \( f = g \circ h \) is semantically G-invariant. Given the semantic $G$-invariance, for any \( \mathbf{x} \) and \( e \), the semantic representation produced by \( g \) is consistent, i.e., \( g(\mathbf{x}) = g(G(\mathbf{x}, e)) \). Since \( f \) is the composition of \( g \) and \( h \), and \( g \) produces consistent outputs for \( \mathbf{x} \) and \( G(\mathbf{x}, e) \), it follows that \( h(g(\mathbf{x})) = h(g(G(\mathbf{x}, e))) \). Consequently, \( f(\mathbf{x}) = f(G(\mathbf{x}, e)) \), establishing that \( f \) is G-invariant. This logical sequence demonstrates that semantic $G$-invariance necessitates $G$-invariance.

Conversely, proving that $G$-invariance does not imply semantic $G$-invariance requires demonstrating a scenario where a predictor is G-invariant without maintaining semantic consistency. Consider a G-invariant predictor \( f = g \circ h \) where \( f(\mathbf{x}) = f(G(\mathbf{x}, e)) \) for all \( \mathbf{x} \) and \( e \). This $G$-invariance does not mandate that the semantic component \( g \) of the predictor treats \( \mathbf{x} \) and \( G(\mathbf{x}, e) \) identically. It is possible that \( g(\mathbf{x}) \neq g(G(\mathbf{x}, e)) \), yet the subsequent processing by \( h \) compensates for this difference, resulting in \( f(\mathbf{x}) = f(G(\mathbf{x}, e)) \). This scenario illustrates that a predictor can be G-invariant without being semantically G-invariant, as the semantic representations \( g(\mathbf{x}) \) and \( g(G(\mathbf{x}, e)) \) may differ.

In summary, while semantic $G$-invariance ensures $G$-invariance due to the inherent requirement of semantic consistency across domain transformations, the broader concept of $G$-invariance does not necessitate such semantic consistency. Therefore, a system or model that is G-invariant may not necessarily exhibit semantic $G$-invariance, highlighting a nuanced distinction between these two forms of invariance.
\end{proof}

\begin{customthm}{2}[A Limitation of $G$-invariance for \sysname{}]
Under the above assumptions, suppose we consider the application of either a density-based OOD detector, as delineated in Equation~(\ref{eq:DDU}), or an energy-based OOD detector, referenced in \cite{liu2020energy}. If the semantic $G$-invariance constraint within the \sysname{} framework (\ref{eq:SODIUM}) is substituted with a $G$-invariance constraint, there exists an optimal G-invariant solution \( \tilde{\bm{\theta}} \) that ranks all ID instances at or above the OOD instances in terms of OOD scoring within any test domain \( e' \) not included in \( \mathcal{E}_{\text{train}} \). Such a ranking leads to suboptimal OOD detection performance, highlighting a significant limitation of relying solely on $G$-invariance in the \sysname{} context.
\end{customthm}

\begin{proof}
We first consider the energy-based OOD detector.  Let $\hat{\bm{\theta}} = (\hat{\bm{\phi}}, \hat{\bm{\psi}})$ represent one of the optimal solutions to the revised \sysname{} problem, namely,  \sysname{}-GI, by replacing the semantic $G$-invariance constraint with the $G$-invariance constraint.  

Let $\bar{\bf f}_{\bm \theta}$ be the logit-output of the predictor ${\bf f}_{\bm \theta}$: ${\bf f}_{\bm \theta}({\bf x}) = \text{softmax}(\bar{\bf f}_{\bm \theta}({\bf x}))= [\frac{e^{\bar{f}_{{\bm \theta}, 1}({\bf x})}}{\sum_{i=1}^K e^{\bar{f}_{{\bm \theta}, i}({\bf x})}}, \cdots, \frac{e^{\bar{f}_{{\bm \theta}, K}({\bf x})}}{\sum_{i=1}^K e^{\bar{f}_{{\bm \theta}, i}({\bf x})}}]^T$. 

For energy-based detection, the negative energy of the predictor ${\bf f}_{\hat{\bm \theta}}$ is used as the OOD scoring function: 
\begin{eqnarray}
    o({\bf x}; {\bf f}_{\hat{\bm \theta}}) = - E({\bf x}; \bar{\bf f}_{\hat{\bm \theta}}) = T \cdot \log \sum_{i=1}^K e^{\bar{f}_{\hat{\bm \theta}, i}({\bf z})/T},
\end{eqnarray}
where $T$ is a predefined temperature parameter. 

Due to the UAP assumption of the predictor $\bar{\bf f}_{\bm \theta}$, for any $r\in \mathbb{R}$, there exists a G-invariant optimal solution $\tilde{\bm \theta}_r$  to the \sysname{}-GI problem, such that 
%\jia{The right hand side of Eq.(10) should be ${\bf f}_{\tilde{\bm \theta}_r}$ }
\begin{eqnarray}
\bar{\bf f}_{\tilde{\bm \theta}_r}({\bf x}) = 
    \begin{cases} 
    \bar{\bf f}_{\hat{\bm \theta}}({\bf x}) + r & \text{if } {\bf x}\sim \mathbb{P}_{ID}(X^{e^\prime})  \\ 
    \bar{\bf f}_{\hat{\bm \theta}}({\bf x}^e) & \text{otherwise}.
    \end{cases}    
\end{eqnarray}

It suffices to prove that, ${\bf f}_{\tilde{\bm \theta}_r}({\bf x}^e) = {\bf f}_{\hat{\bm \theta}}({\bf x}^e)$ , $\forall e\in \mathcal{E}_{\text{\text{all}}}$. By the definition of ${\bf f}_{\tilde{\bm \theta}_r}({\bf x})$, this equality holds for each ${\bf x}\nsim \mathbb{P}_{ID}(X^{e^\prime})$.  For each ${\bf x}^{e^\prime} \sim \mathbb{P}_{ID}(X^{e^\prime})$,  we have that 
\begin{align}
   {\bf f}_{\tilde{\bm \theta}_r}({\bf x}^{e^\prime}) &= \text{softmax}(\bar{\bf f}_{\tilde{\bm \theta}_r}({\bf x}^{e^\prime})) \\
   &= [\frac{e^{\bar{f}_{\tilde{\bm \theta}, 1}({\bf x})}}{\sum_{i=1}^K e^{\bar{f}_{\tilde{\bm \theta}, i}({\bf x})}}, \cdots, \frac{e^{\bar{f}_{\tilde{\bm \theta}, K}({\bf x}^{e^\prime})}}{\sum_{i=1}^K e^{\bar{f}_{\tilde{\bm \theta}, i}({\bf x}^{e^\prime})}}]^T \\
   &= [\frac{e^{\bar{f}_{\hat{\bm \theta}, 1}({\bf x}^{e^\prime})}\cdot e^r}{\sum_{i=1}^K e^{\bar{f}_{\hat{\bm \theta}, i}({\bf x}^{e^\prime})}\cdot e^r}, \cdots, \frac{e^{\bar{f}_{\hat{\bm \theta}, K}({\bf x}^{e^\prime})}\cdot e^r}{\sum_{i=1}^K e^{\bar{f}_{\hat{\bm \theta}, i}({\bf x}^{e^\prime})}\cdot e^r}]^T \\
&= [\frac{e^{\bar{f}_{{\bm \theta}, 1}({\bf x}^{e^\prime})}}{\sum_{i=1}^K e^{\bar{f}_{{\bm \theta}, i}({\bf x}^{e^\prime})}}, \cdots, \frac{e^{\bar{f}_{{\bm \theta}, K}({\bf x}^{e^\prime})}}{\sum_{i=1}^K e^{\bar{f}_{{\bm \theta}, i}({\bf x}^{e^\prime})}}]^T \\
&= {\bf f}_{\hat{\bm \theta}}({\bf x}^{e^\prime}). 
\end{align}
We can then identify the relation between the energy-based OOD scoring functions $o({\bf x}; \bar{\bf f}_{\tilde{\bm \theta}})$ and $o({\bf x}; \bar{\bf f}_{\hat{\bm \theta}})$ as follows: 
\begin{align}
o({\bf x}; \bar{\bf f}_{\tilde{\bm \theta}}) = - E({\bf x}; \bar{\bf f}_{\tilde{\bm \theta}}) &= T \cdot \log \sum_{i=1}^K e^{\bar{f}_{\tilde{\bm \theta}, i}({\bf x})/T} \\
&= T \cdot \log (\sum_{i=1}^K e^{\bar{f}_{\hat{\bm \theta}, i}({\bf x})/T} \cdot e^{\frac{r}{T}}) \\
&=  T \cdot \log \sum_{i=1}^K e^{\bar{f}_{\hat{\bm \theta}, i}({\bf x})/T} + r \\
&= -E({\bf x}; \bar{\bf f}_{\hat{\bm \theta}}) + r \\
&= o({\bf x}; \bar{\bf f}_{\hat{\bm \theta}}) + r. 
\end{align}
Therefore, as the OOD data distribution $\mathbb{P}_{OD}(X_O^{e^\prime})$ is bounded, there exists a sufficiently large positive value of $r$  such that, for each ${\bf x}^{e^\prime}\sim \mathbb{P}_{IN}(X^{e^\prime})$, we have $o({\bf x}^{e^\prime}; \bar{\bf f}_{\tilde{\bm \theta}}) = o({\bf x}^{e^\prime}; \bar{\bf f}_{\hat{\bm \theta}}) + r\ge \max_{{\bf x} \sim \mathbb{P}_{OD}(X_O^{e^\prime})} o({\bf x}; \bar{\bf f}_{\tilde{\bm \theta}})$, where by definition $\bar{\bf f}_{\hat{\bm \theta}}({\bf x}^e) = \bar{\bf f}_{\hat{\bm \theta}}({\bf x}^e)$, when $e\nsim \mathbb{P}_{ID}(X^{e^\prime})$.  We conclude that all the ID instances are ranked higher than OOD instances in a test domain $e\in \mathcal{E}_{\text{\text{all}}}\setminus \mathcal{E}_{\text{train}}$  by the energy-based OOD detector. 

In the following, we consider the density-based OOD detector as specified in Equation~(\ref{eq:DDU}). Let $d_{\hat{\bm \phi}}(\cdot)$ denote the density function estimated based on the training set $\mathcal{D}$ in the semantic representation space ${\bf g}_{\hat{\bm \phi}}$. The density function of the OOD data distribution $\mathbb{P}_{OOD}({\bf g}_{\hat{\bm \phi}}(X_O^{e}))$ is assumed available and denoted as $d_{\hat{\bm \phi}}({\bf g}_{\hat{\bm \phi}}({\bf x}))$. The OOD scoring function is defined based on the density function: $o({\bf x}, {\bf g}_{\hat{\bm \phi}}) = -d_{\hat{\bm \phi}}({\bf g}_{\hat{\bm \phi}}({\bf x}))$.  

Let $\hat{\bm{\theta}} = (\hat{\bm{\phi}}, \hat{\bm{\psi}})$ represent one of the optimal solutions to the \sysname{}-GI problem. Let the OOD scoring function $o({\bf x}, {\bf g}_{\bm \phi})$ denote a density model estimated based on the training instances $\mathcal{D}$ in the semantic representation space encoded by ${\bf g}_{\bm \phi}$. 

For each feature vector ${\bf x}\in \mathcal{X}$ and each specification of ${\bm \theta}$, let ${\bf p}_{{\bm \theta}, {\bf x}}$ denote the  probability vector of ${\bf x}$ predicted by the predictor ${\bf f}_{\bm \theta}$: ${\bf p}_{{\bm \theta}, {\bf x}} = {\bf f}_{\bm \theta}({\bf x})$.  Due to the assumptions that the predictor ${\bf f}_{\bm \theta}$  satisfies UAP, the OOD data distribution $\mathbb{P}_{OOD}(X_O^{e^\prime})$ is bounded in the test domain $e^\prime$, and the inverse image of the classifier ${\bf h}_{\bm \psi}$ is unbounded, there exists a semantic feature vector ${\bf z}_{{\bm \theta}, {\bf x}}\in \bf{h}_{\tilde{\bm \psi}}^{-1}({\bf p}_{{\bm \theta}, {\bf x}})$, such that $d_{\bm \phi}({\bf z}_{{\bm \theta}, {\bf x}}) = 0$.  

Therefore, there exists a G-invariant optimal solution $\tilde{\bm \theta} = (\tilde{\bm \phi}, \tilde{\bm \psi})$  to the \sysname{}-GI problem, such that 
\begin{eqnarray}
{\bf g}_{\tilde{\bm \phi}}({\bf x}) = 
    \begin{cases} 
    {\bf z}_{\tilde{\bm \theta}, {\bf x}} & \text{if } {\bf x}\sim \mathbb{P}_{ID}(X^{e^\prime})  \\ 
    {\bf g}_{\hat{\bm \phi}}({\bf x}) & \text{otherwise}.
    \end{cases}    
\end{eqnarray}
We must highlight that the density function $d_{\hat{\bm \phi}}(\cdot)$ is estimated based on the semantic vectors of the training instances in $\mathcal{D}$,  which are extracted by ${\bf g}_{\hat{\bm \phi}}({\bf x})$, based on the above specification of $\tilde{\bf \theta}$. For this reason, when we discuss the density function below, we always use $\hat{\bm \phi}$ to represent the density function $d_{\hat{\bm \phi}}(\cdot)$. Then, for each ${\bf x}^{e^\prime}\sim \mathbb{P}_{ID}(X^{e^\prime})$, we have that $o({\bf x}^{e^\prime}, {\bf g}_{\tilde{\bm \phi}}) = -d_{\hat{\bm \phi}}({\bf g}_{\tilde{\bm \phi}}({\bf x}^{e^\prime})) = -d_{\hat{\bm \phi}}({\bf z}_{\tilde{\bm \theta}, {\bf x}}) = 0\ge \min_{{\bf x}_O^{e^\prime}\sim \mathbb{P}_{OOD}(X_O^{e^\prime})} -d_{\hat{\bm \phi}}({\bf x}_O^{e^\prime})$. 
We conclude that all the ID instances are ranked higher than OOD instances in a test domain $e\in \mathcal{E}_{\text{\text{all}}}\setminus \mathcal{E}_{\text{train}}$  by the density-based OOD detector. 
\end{proof}

\begin{customthm}{3}[Effectiveness of semantic $G$-invariance]
In the context of the same assumptions and framework outlined in Proposition~\ref{prop:G-invariance-limitation}, substituting the $G$-invariance constraint with semantic $G$-invariance within the \sysname{} problem~(\ref{eq:SODIUM}) guarantees that every optimal solution achieves optimal OOD detection performance. 
Specifically, it ensures that ID instances are consistently ranked below OOD instances across all test domains $e \in \mathcal{E}_{\text{\text{all}}} \setminus \mathcal{E}_{\text{train}}$, thereby enhancing the effectiveness of OOD detection.
\end{customthm}

% Under the same assumptions and settings as in Proposition ?, replacing the $G$-invariance constraint with semantic $G$-invariance in the \sysname{} problem ensures that any optimal solution ranks all ID instances lower than OOD instances in any test domain $e \in \mathcal{E}_{\text{\text{all}}} \setminus \mathcal{E}_{\text{train}}$.
% \begin{proof}[Proof Sketch]
% The proof starts with an optimal solution $\tilde{\bm \theta}$ that adheres to semantic $G$-invariance, preserving semantic features across domain transformations. This preservation is crucial for maintaining the separability of ID and OOD instances, as ensured by the $R_{\text{OOD}}$ regularization term. It then leverages the availability of the ID data distribution's density function in the semantic space, showing that ID instances have positive density scores while OOD instances score zero. semantic $G$-invariance guarantees this distinction holds in all domains, including test domains not seen during training, thus ensuring the effective separation of ID and OOD instances based on their density scores. 
% \end{proof}
\begin{proof}
%Consider an ID data distribution $\mathbb{P}_{IN}(X, Y)$ and a domain transformation model $G$. 
Let $\hat{\bm{\theta}} = (\hat{\bm{\phi}}, \hat{\bm{\psi}})$ be any optimal solution to the \sysname{} problem that minimizes the expected risk across domains $\mathcal{E}_{\text{\text{all}}}$ and satisfies the $R_{\text{OOD}}$ regularization term under semantic $G$-invariance. This implies:
\begin{equation}
    \mathbf{g}_{\hat{\bm{\phi}}}(\mathbf{x}) = \mathbf{g}_{\hat{\bm{\phi}}}(G(\mathbf{x}, e)), \quad \forall \mathbf{x} \in \mathcal{X}, \forall e \in \mathcal{E}_{\text{\text{all}}},
\end{equation}
ensuring the preservation of semantic features across domain transformations.

Given the separability of $\mathbb{P}_{IN}(X)$ and $\mathbb{P}_{OOD}(X_O)$, the $R_{\text{OOD}}$ regularization guarantees separability in the logit-output space of ${\bf f}_{\hat{\bm{\theta}}}$. Consequently, this separability must also exist in the semantic representation space ${\bf g}_{\hat{\bm{\phi}}}$, as the classifier ${\bf h}_{\hat{\bm{\psi}}}$ maps semantic representations to logit-outputs.

The density function of the ID data distribution $\mathbb{P}_{ID}({\bf g}_{\hat{\bm \phi}}(X^{e}))$ is assumed to be available for each training domain $e\in \mathcal{E}_{\text{train}}$. Due to the separability between the OOD and ID data distributions in the semantic space for each training domain $e \in \mathcal{E}_{\text{train}}$, the density function $d_{\hat{\bm{\phi}}}({\bf g}_{\hat{\bm{\phi}}}({\bf x}^{e}))$ in the semantic space is positive for ID instances and zero for OOD instances:
\begin{align}
    d_{\hat{\bm{\phi}}}({\bf g}_{\hat{\bm{\phi}}}({\bf x}^{e})) &> 0, \quad \forall {\bf x}^e \in \mathbb{P}_{ID}(X^e), \\
    d_{\hat{\bm{\phi}}}({\bf g}_{\hat{\bm{\phi}}}({\bf x}^{e}_O)) &= 0, \quad \forall {\bf x}^e_O \in \mathbb{P}_{OOD}(X^e_O).
\end{align}

semantic $G$-invariance ensures that for any ${\bf x}^{e^\prime} \sim \mathbb{P}_{ID}(X^{e^\prime})$ in a test domain, there exists a corresponding ${\bf x}^e \sim \mathbb{P}_{ID}(X^e)$ in a training domain such that:
\begin{equation}
    {\bf g}_{\hat{\bm{\phi}}}({\bf x}^{e^\prime}) = {\bf g}_{\hat{\bm{\phi}}}(G({\bf x}, e^\prime)) = {\bf g}_{\hat{\bm{\phi}}}(G({\bf x}, e)) = {\bf g}_{\hat{\bm{\phi}}}({\bf x}^{e}) > 0.
\end{equation}
Similarly, for OOD instances in the test domain, the density score remains zero:
\begin{equation}
    {\bf g}_{\hat{\bm{\phi}}}({\bf x}_O^{e^\prime}) = {\bf g}_{\hat{\bm{\phi}}}(G({\bf x}_O, e^\prime)) = {\bf g}_{\hat{\bm{\phi}}}(G({\bf x}_O, e)) = {\bf g}_{\hat{\bm{\phi}}}({\bf x}_O^{e}) = 0.
\end{equation}

Thus, under semantic $G$-invariance, all ID instances in a test domain $e^\prime$ are guaranteed to have a positive density score, ensuring they are ranked lower than OOD instances with a density score of zero. This concludes the proof that semantic $G$-invariance effectively maintains the separability of ID and OOD instances across domain transformations in the \sysname{} framework.
\end{proof}

\subsection{Detailed Experimental Settings}
\label{sec:experiment_setting_details}
\subsubsection{Environment and Experiment Setup}
The environment we used: Python: 3.9.13, PyTorch: 1.12.1, Torchvision: 0.13.1, CUDA: 11.6, CUDNN: 8302, NumPy: 1.23.1, PIL: 9.2.0.
Experiment setup: Our experimental framework, tailored for semantic OOD detection in unseen domains, deviates from the conventional setups for OOD detection and domain generalization. Uniquely, in our configuration, the OOD samples are always sourced from an unseen test domain. For each dataset, we designated one class as OOD and iterate our experiments with different randomly chosen OOD classes until a minimum of 40\% of classes have been designated as OOD. To further mitigate the impact of randomness, each set of experiments is conducted in two separate trials with different seeds. The results reported in the paper represent mean and standard error across these trials and all OOD class choices. Furthermore, given the multiple OOD detection methods evaluated in this study, and in an effort to present the results in a concise manner, for the OOD detection performance we report the averaged values across all test domains unless specified otherwise.

\subsubsection{Model Selection} Commonly used model selection strategies include training-domain validation, leave-one-domain-out cross-validation, and test-domain validation. Training-domain validation holds out a portion of the training data as the validation set, but essentially, it assumes that the test domain adheres to the same distribution as the training domains, which contradicts the concept of domain generalization. Test-domain validation uses part of the test set for model selection, but in practice, we typically lack any information about the target domain. Leave-one-domain-out cross-validation utilizes a held-out training domain as a validation set. This strategy presumes that training and test domains follow a meta-distribution over domains, which more closely aligns with real-world scenarios.

Considering both the experimental framework and the practical considerations related to experiment execution time, we carried out a random search of 20 trials over the hyperparameter distribution for each algorithm and test domain. The detailed hyperparameters space and their corresponding default values are specified in Table~\ref{tab:hyperparamesters}, other hyperparameters (\textit{e.g.,} learning rate, weight decay, \textit{etc.}) that are not listed in this table are left unchanged from the DomainBed framework.

% \subsubsection{Hyperparameter Search}
% Considering both the experimental framework and the practical considerations related to experiment execution time, we carried out a random search of 20 trials over the hyperparameter distribution for each algorithm and test domain. To be more specific, we partitioned the data from each domain into an 80-20 split. The larger portion was designated for training and evaluation, while the smaller was used for hyperparameter selection.
% The detailed hyperparameters space and their corresponding default values are specified in Table~\ref{tab:hyperparamesters}, other hyperparameters (\textit{e.g.,} learning rate, weight decay, \textit{etc.}) that are not listed in this table are left unchanged from the DomainBed framework.

\subsubsection{Datasets}
In our study, we assess the performance of our model on four popular datasets widely used in the field of domain generalization (DG): \textsc{ColoredMNIST} (3 domains, 70,000 samples, 2 classes), \textsc{PACS} (4 domains, 9,991 samples, 7 classes), and \textsc{VLCS} (4 domains, 10,729 samples, 5 classes).

\textsc{ColoredMNIST} is a variant of the popular MNIST dataset of handwritten digits. It introduces color as a spurious feature, thereby creating three distinct domains for evaluating domain generalization capabilities. The three domains: [+90\%, +80\%, -90\%] are characterized by different levels of digit color and label correlations. The original 10 digits are split into two classes: digits from 0-4 are categorized with label 0, while digits from 5-9 receive label 1. Note that there is a 25\% manually injected error in the binary labels, which makes \textsc{ColoredMNIST} challenging for the domain generalization task.

\textsc{PACS} dataset comprises images sourced from four discrete domains: Art Painting (A), Cartoon (C), Photo (P), and Sketch (S). Each domain offers a wide array of images showcasing diverse objects, scenes, and IDividuals. These images are categorized into seven different categories, namely dog, elephant, giraffe, guitar, horse, house, and person.

\textsc{VLCS} is a collection of four well-established datasets
commonly used in computer vision research: Caltech101 (C), LabelMe (L), SUN09 (S), and VOC2007 (V). These datasets, when brought
together, offer an extensive variety of images across diverse
contexts and subjects, making them an ideal test bed for assessing
domain generalization capabilities. These images are categorized into five classes: person, dog, chair, car, and bird.

\textsc{TerraIncognita} dataset amalgamates wildlife images hailing from a variety of discrete locations, each distinctly labeled as L100, L38, L43, and L46. This rich compilation showcases a diverse array of fauna captured in their natural habitats. Encompassing a multitude of species, the dataset is meticulously categorized into an array of classes, namely bird, bobcat, cat, coyote, dog, opossum, rabbit, raccoon, and squirrel. Tailored for the domain of computer vision, particularly in the challenging context of domain generalization, the TerraIncognita dataset serves as an exemplary foundation for models aiming to achieve robust performance across variegated environmental conditions.

Some examples of \textsc{ColoredMNIST}, \textsc{PACS}, and \textsc{VLCS} are shown in Figure~\ref{fig:data-example}.

\begin{figure*}
\centering
\begin{subfigure}{.3\linewidth}
  \centering
  \includegraphics[width=.9\linewidth]{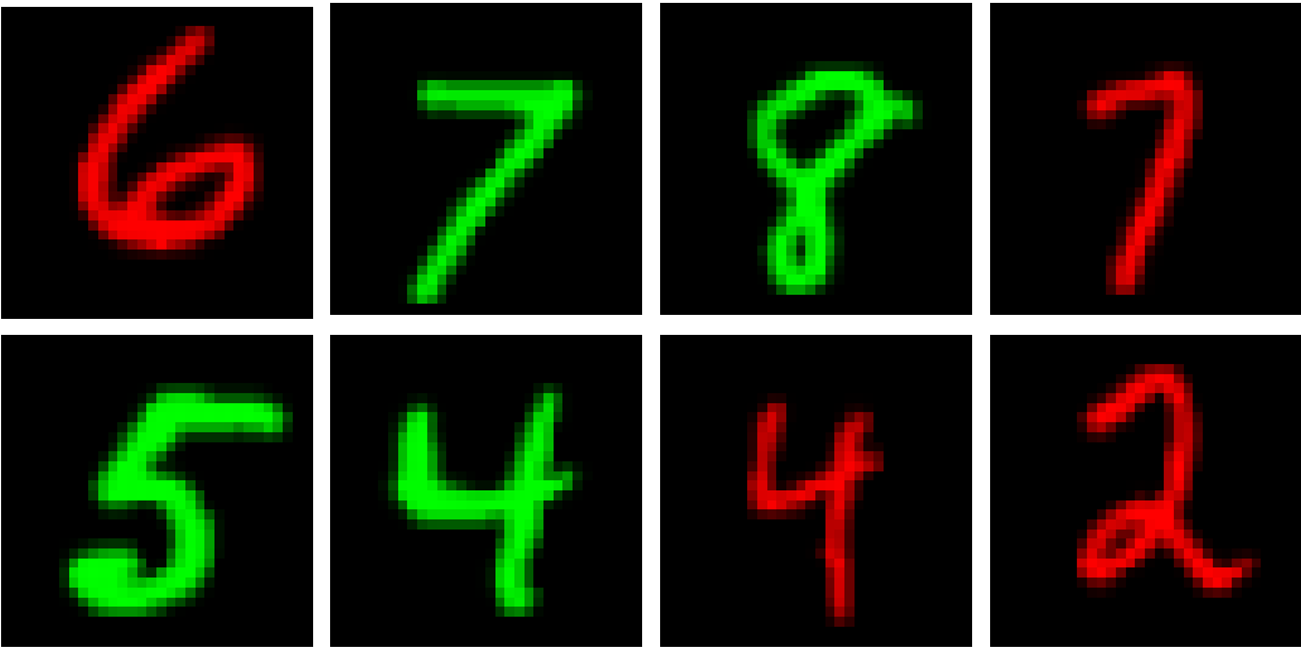}
  \caption{\textsc{ColoredMNIST}}
  \label{fig:coloredmnist}
\end{subfigure}%
\begin{subfigure}{.34\linewidth}
  \centering
  \includegraphics[width=.9\linewidth]{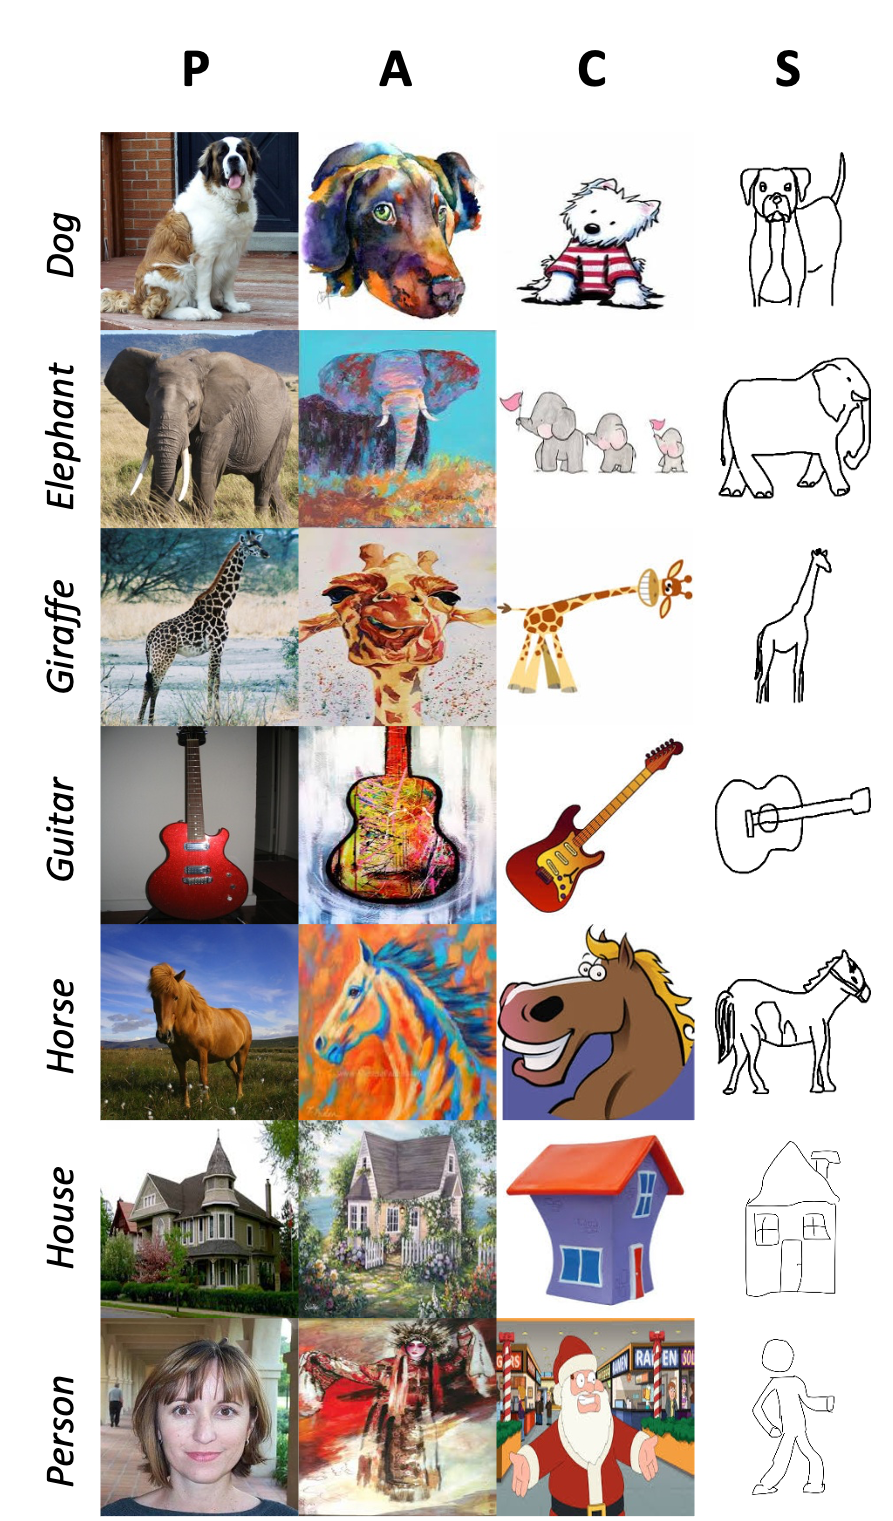}
  \caption{\textsc{PACS}}
  \label{fig:pacs}
\end{subfigure}
\begin{subfigure}{.34\textwidth}
  \centering
  \includegraphics[width=1\linewidth]{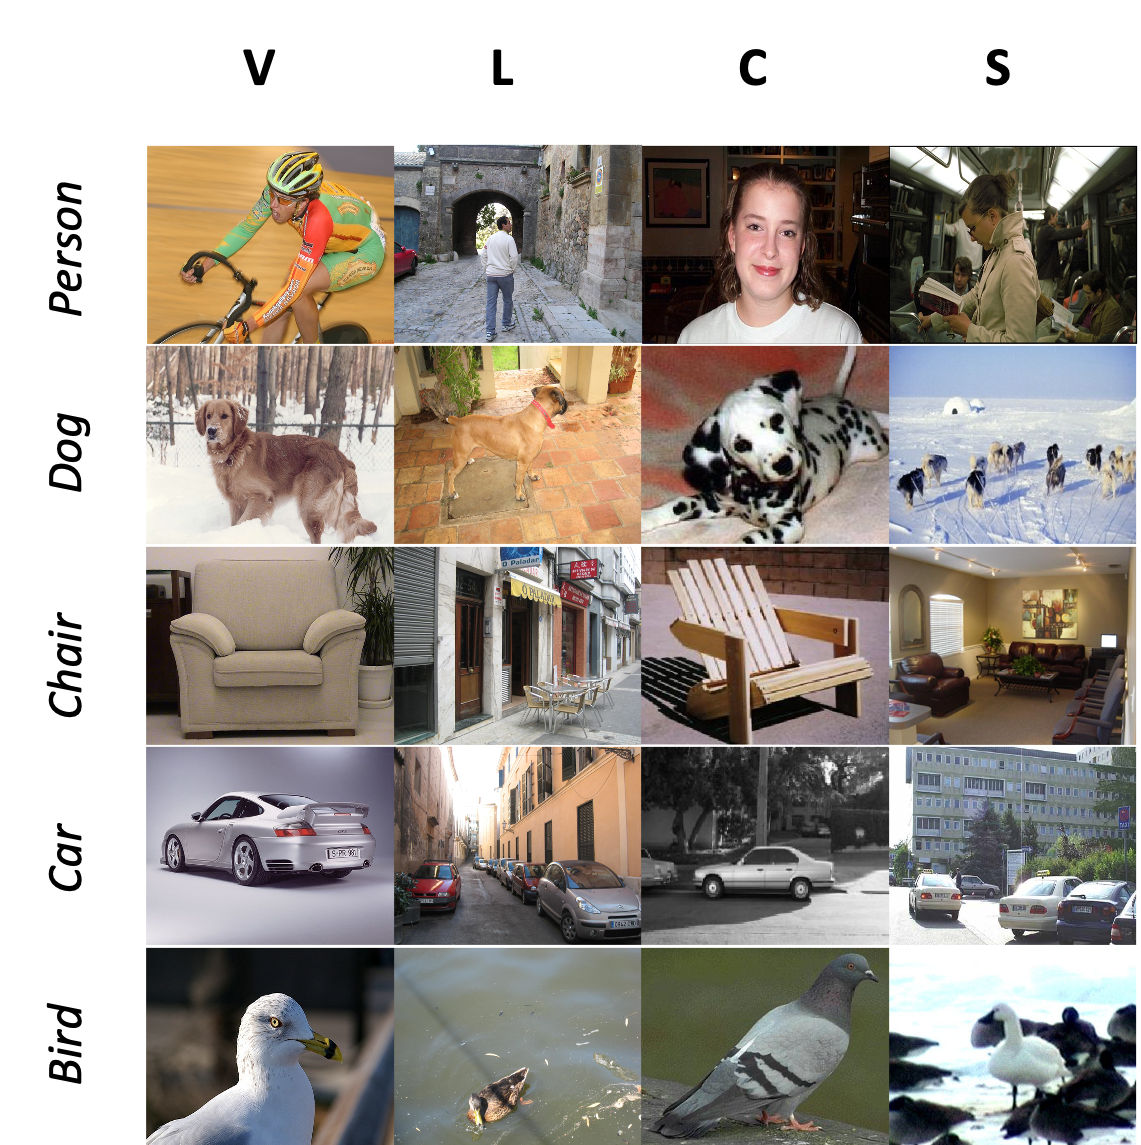}
  \caption{\textsc{VLCS}}
  \label{fig:vlcs}
\end{subfigure}
\caption{Samples from each dataset. (a) \textsc{ColoredMNIST} domains are different levels of digit color and label correlation: +90\%, +80\%, and -90\%; (b) \textsc{PACS} domains are: Photo (P), Art Painting (A), Cartoon (C), and Sketch (S); (c) \textsc{VLCS} domains are: VOC2007 (V), LabelMe (L), Caltech101 (C), and SUN09 (S).}
\label{fig:data-example}
\end{figure*}

\subsubsection{Baselines}
In our comparative analysis, we evaluated the performance of \sysname{} against four widely recognized domain generalization methods: ERM \cite{vapnik1999nature}, IRM \cite{arjovsky2019invariant}, Mixup \cite{yan2020improve}, and MBDG \cite{robey2021model}. Additionally, \sysname{} was compared with five SOTA open-set domain generalization baselines: DAML \cite{shu2021open}, MEDIC \cite{wang2023generalizable}, SCONE \cite{bai2023feed}, EDir-MMD and EDst-MMD \cite{noguchi2023simple}. All these experiments were conducted within the DomainBed \cite{gulrajani2020search} framework, ensuring a consistent and standardized assessment across different methods.

\subsubsection{OOD Detection Methods}
To evaluate the performance of OOD detection, we employ four widely-used OOD detection methods: Maximum Softmax Probability (MSP) \cite{hendrycks2016baseline}, Energy-based Out-of-Distribution Detection (Energy) \cite{liu2020energy}, Deep Deterministic Uncertainty (DDU) \cite{mukhoti2023deep}, and One-Class Support Vector Machine (OCSVM) \cite{scholkopf1999support}. Each of these methods brings its unique approach to the problem, leveraging different aspects of the neural network's feature characteristics. As such, they each have their inherent strengths and potential limitations, providing us with a comprehensive understanding of our model's OOD detection performance.

MSP (Maximum Softmax Probability) uses the softmax outputs of neural networks to identify OODs. Based on the assumption that neural networks are less confident when classifying OOD samples, hence, samples with lower maximum softmax probabilities are categorized as OOD.

Energy (Energy-based Out-of-Distribution Detection) employs the output 'energies' of samples to detect OOD, with higher energy values IDicating OOD samples. In comparison to MSP, Energy scores provide a closer representation of the input's probability density. As a result, they are less susceptible to the overconfidence issue.

DDU (Deep Deterministic Uncertainty) detects OODs through estimated epistemic uncertainty (model uncertainty). The epistemic uncertainty of input is estimated by examining their feature-space density to the training data. Specifically, a per-class Gaussian mixture model (GMM) is fitted in the feature space, and at test time, the GMM is used to evaluate the test sample's marginal likelihood of its hidden representations in the feature space. 

OCSVM (One-Class SVM) is a machine learning method specifically designed for anomaly detection. Unlike traditional SVMs that differentiate between two classes, OCSVM aims to identify patterns that conform to what it has seen during training (the "one class") and flag anything different as an outlier or anomaly. It achieves this by trying to maximize the distance between the data and the origin in the feature space, and then determining a decision boundary around the data. Anything that falls outside this boundary in the feature space is considered an anomaly. OCSVM is particularly useful in scenarios where "normal" data is abundant, but "anomalous" data is scarce or unavailable during training.

\subsubsection{Evaluation Metrics}
To evaluate domain generalization performance, we simply report the classification accuracy. Meanwhile, to evaluate OOD detection performance, we use AUROC (Area Under the Receiver Operating Characteristic Curve) and AUPR (Area Under the Precision-Recall
Curve). AUROC is a commonly used metric for evaluating the effectiveness of binary classification models. It measures the model's capacity to differentiate between positive and negative classes by computing the area under the ROC curve. This value can range from 0 to 1, with a perfect model having an AUROC of 1 and a random model having an AUROC of 0.5. The AUPR is a metric used to evaluate the performance of a classification model, especially in imbalanced datasets where one class significantly outnumbers the other. The precision-recall curve plots precision against recall for different threshold values. The AUPR calculates the area under this curve, providing a single value that captures the model's ability to correctly classify the positive class across various thresholds. A higher AUPR value IDicates better model performance, with a maximum value of 1. In cases of imbalanced datasets, AUPR is often preferred over the more common AUROC because it focuses specifically on the performance with respect to the positive, or minority class. In the paper, the AUPR values we reported are the AUPR-out which treats OODs as positive samples.
Note that the results reported in the paper are the mean and standard error across trials and all OOD class choices. And for the OOD detection performance evaluation, the AUROC and AUPR values are further averaged across all test domain selections to save space.

\subsection{ColoredMNIST Experimental Results}
\label{sec:coloredmnist_experiment_results}

The \textsc{ColoredMNIST} dataset, particularly the "-90\%" domain, posed significant challenges for standard domain generalization baselines, as detailed in Table~\ref{tab:accuracy-summary}, Table~\ref{tab:ood-details-cmnist-auroc} and Table~\ref{tab:ood-details-cmnist-aupr}. These baselines exhibited notably low classification accuracy, AUROC, and AUPR in the "-90\%" test domain. This underperformance primarily originates from a 25\% intentional label error rate and a pronounced correlation between digit color and label. When trained on the +90\% and +80\% domains, which exhibit strong positive color-label correlations, these networks struggle to adapt to the reversed correlation in the "-90\%" test domain.

Conversely, \sysname{} adeptly handles both mislabeling and inverse correlation issues in the \textsc{ColoredMNIST} dataset. This success is achieved through the application of $G$-invariance against random variations generated by the transformation model, coupled with the label-agnostic semantic OOD detection regularization, $R_{\text{OOD}}$. In the \textsc{ColoredMNIST} context, \sysname{} attained an average AUROC of \num{77.83} and an average AUPR of \num{53.14}, surpassing the next best baseline method by 18.93\% and 40.22\% respectively. Additionally, in the +90\% and +80\% test domains, \sysname{} matched the classification accuracy of the leading baseline (MBDG) and notably outperformed other baselines in the -90\% test domain.

\subsection{Detailed Experimental Results}
\label{sec:experiment_details}

\begin{table*}[!t]
\centering
\setlength\tabcolsep{5pt}
\scriptsize
\caption{Performance comparison for AUPR against domain generalization baselines.}
\label{tab:aupr}
\begin{tabular}{c|l|c|c|c|c}
\toprule
Data & Methods & OCSVM & DDU & MSP & Energy \\
\midrule
\parbox[t]{2mm}{\multirow{5}{*}{\rotatebox[origin=c]{90}{\textsc{\scriptsize CMNIST}}}} 
& ERM & 10.72 $\pm$ 0.38 & 09.13 $\pm$ 0.10 & 09.83 $\pm$ 0.39 & 10.47 $\pm$ 0.04 \\
& IRM & 11.15 $\pm$ 0.10 & 09.42 $\pm$ 0.61 & 10.52 $\pm$ 1.07 & 10.14 $\pm$ 0.65 \\
& Mixup & 10.94 $\pm$ 0.75 & 09.09 $\pm$ 0.04 & 10.43 $\pm$ 0.62 & 09.97 $\pm$ 0.36 \\
& MBDG & 14.14 $\pm$ 1.74 & 08.24 $\pm$ 0.27 & 14.17 $\pm$ 2.52 & 15.16 $\pm$ 2.58 \\
& \sysname{} (ours) & \textbf{55.28} $\pm$ 0.25 & \textbf{42.47} $\pm$ 0.89 & \textbf{57.43} $\pm$ 0.35 & \textbf{57.37} $\pm$ 0.36 \\
\midrule
\parbox[t]{2mm}{\multirow{5}{*}{\rotatebox[origin=c]{90}{\textsc{\scriptsize PACS}}}} 
& ERM & 19.87 $\pm$ 0.92 & 25.06 $\pm$ 3.56 & 32.64 $\pm$ 3.44 & 38.96 $\pm$ 3.36 \\
& IRM & 23.84 $\pm$ 3.22 & 22.28 $\pm$ 3.58 & 35.20 $\pm$ 7.45 & 42.14 $\pm$ 7.63 \\
& Mixup & 17.56 $\pm$ 5.11 & 33.54 $\pm$ 2.46 & 32.70 $\pm$ 6.77 & 35.22 $\pm$ 7.11 \\ 
& MBDG & 22.03 $\pm$ 1.90 & 22.39 $\pm$ 5.24 & 31.93 $\pm$ 4.38 & 36.34 $\pm$ 4.95 \\ 
& \sysname{} (ours) & \textbf{43.37} $\pm$ 0.66 & \textbf{57.30} $\pm$ 0.60 & \textbf{57.26} $\pm$ 0.51 & \textbf{57.70} $\pm$ 0.50 \\
\midrule
\parbox[t]{2mm}{\multirow{5}{*}{\rotatebox[origin=c]{90}{\textsc{\scriptsize VLCS}}}} 
& ERM & 08.82 $\pm$ 2.25 & 21.46 $\pm$ 7.57 & 24.52 $\pm$ 11.83 & 27.63 $\pm$ 12.34 \\
& IRM & 09.69 $\pm$ 2.35 & 20.75 $\pm$ 8.00 & 23.73 $\pm$ 11.54 & 27.82 $\pm$ 12.28 \\
& Mixup & 10.31 $\pm$ 2.95 & 26.63 $\pm$ 4.60 & 21.60 $\pm$ 10.69 & 26.14 $\pm$ 10.55 \\
& MBDG & 08.34 $\pm$ 2.53 & 18.66 $\pm$ 0.91 & 15.92 $\pm$ 05.25 & 21.16 $\pm$ 07.42 \\
& \sysname{} (ours) & \textbf{39.42} $\pm$ 3.43 & \textbf{48.73} $\pm$ 1.73 & \textbf{47.40} $\pm$ 02.60 & \textbf{48.04} $\pm$ 02.23 \\
\midrule
\parbox[t]{2mm}{\multirow{5}{*}{\rotatebox[origin=c]{90}{\textsc{\scriptsize Terra}}}} 
& ERM & 12.56 $\pm$ 2.53 & 17.32 $\pm$ 5.52 & 16.63 $\pm$ 4.36 & 18.43 $\pm$ 4.43 \\
& IRM & 13.97 $\pm$ 5.21 & 17.95 $\pm$ 6.43 & 18.52 $\pm$ 5.83 & 21.05 $\pm$ 6.46 \\
& Mixup & 14.08 $\pm$ 6.62 & 15.99 $\pm$ 5.44 & 19.22 $\pm$ 6.25 & 18.05 $\pm$ 5.74 \\
& MBDG & 13.42 $\pm$ 4.33 & \textbf{20.20} $\pm$ 6.41 & 16.55 $\pm$ 3.76 & 17.07 $\pm$ 3.73 \\
& \sysname{} (ours) & \textbf{15.08} $\pm$ 4.40 & 17.15 $\pm$ 4.89 & \textbf{21.99} $\pm$ 5.65 & \textbf{23.70} $\pm$ 6.02 \\
\bottomrule
\end{tabular}
\end{table*}

Table~\ref{tab:auroc} and Table~\ref{tab:aupr} provide an overview of \sysname{}'s OOD detection performance compared to various domain generalization baselines. Here, AUROC and AUPR values are averaged across all trials, OOD class selections, and test domains. For a detailed evaluation, per-domain results are provided in Tables \ref{tab:ood-details-pacs-auroc}, \ref{tab:ood-details-pacs-aupr}, \ref{tab:ood-details-vlcs-auroc}, \ref{tab:ood-details-vlcs-aupr}, \ref{tab:ood-details-terra-auroc}, and \ref{tab:ood-details-terra-aupr}, with AUROC and AUPR values averaged across trials and OOD class choices for each test domain. \sysname{} consistently outperforms baseline methods in all test domains, particularly in AUPR, where it significantly exceeds baselines. Notably, AUPR values are generally lower than AUROC, highlighting the challenge of accurately detecting semantic OODs in unseen test domains. This is because OODs and ID test samples come from the same test domain, presenting a substantial challenge for an OOD detector to maintain high precision and recall simultaneously. Additionally, Table~\ref{tab:accuracy-summary} shows the ID classification results, where \sysname{} often matches or even exceeds baseline performance, particularly on the \textsc{ColoredMNIST} dataset.

\begin{table*}[!t]
\centering
\scriptsize
\caption{ID Classification Accuracy. All classification accuracy values presented are averaged over all trials and OOD class choices. Top results are highlighted in \textbf{bold}.}
\label{tab:accuracy-summary}
\begin{tabular}{c|l|c|c|c|c|c}
\toprule
\multirow{3}{*}{Data} &  & \multicolumn{5}{c}{\textbf{ID Classification, Accuracy}} \\
\cmidrule{3-7}
& & \multicolumn{5}{c}{Test Domains} \\
\midrule
& Methods & +90\% & +80\% & -90\% & & Avg \\ 
\cmidrule{2-7}
\parbox[t]{2mm}{\multirow{5}{*}{\rotatebox[origin=c]{90}{\textsc{\scriptsize ColoredMNIST}}}} 
& ERM    & 43.91 $\pm$ 3.72 & 49.69 $\pm$ 1.47 & 10.21 $\pm$ 0.26 & & 34.71 \\
& IRM    & 51.63 $\pm$ 1.85 & 59.84 $\pm$ 1.55 & 12.85 $\pm$ 2.15 & & 41.52 \\
& Mixup  & 50.02 $\pm$ 0.77 & 48.85 $\pm$ 1.15 & 10.17 $\pm$ 0.07 & & 36.44 \\
& MBDG   & 68.67 $\pm$ 2.76 & 70.54 $\pm$ 2.91 & 19.16 $\pm$ 3.30 & & 52.87 \\
\cmidrule{2-7}
& \sysname{} (ours)   & \textbf{73.10} $\pm$ 0.37 & \textbf{72.51} $\pm$ 0.44 & \textbf{67.07} $\pm$ 3.17 & & \textbf{70.94} \\
\midrule
& Methods & A & C & P & S & Avg \\
\cmidrule{2-7}
\parbox[t]{2mm}{\multirow{5}{*}{\rotatebox[origin=c]{90}{\textsc{\scriptsize PACS}}}} 
& ERM   & 87.92 $\pm$ 1.60 & 79.36 $\pm$ 1.67 & 96.31 $\pm$ 0.93 & 74.34 $\pm$ 0.37 & 84.48 \\ 
& IRM   & 86.90 $\pm$ 1.31 & 79.22 $\pm$ 1.79 & 95.16 $\pm$ 0.64 & 74.41 $\pm$ 3.07 & 83.92 \\ 
& Mixup & 88.93 $\pm$ 0.91 & 79.80 $\pm$ 1.55 & \textbf{96.82} $\pm$ 0.60 & 74.13 $\pm$ 2.52 & 84.92 \\ 
& MBDG  & 82.67 $\pm$ 0.85 & 72.87 $\pm$ 1.03 & 80.7 $\pm$ 10.87 & \textbf{81.34} $\pm$ 1.53 & 79.40 \\ 
\cmidrule{2-7}
& \sysname{} (ours)  & \textbf{89.64} $\pm$ 1.44 & \textbf{81.31} $\pm$ 2.26 & 96.12 $\pm$ 0.43 & 76.20 $\pm$ 2.18 & \textbf{85.82} \\ 
\midrule
& Methods & C & L & S & V & Avg \\
\cmidrule{2-7}
\parbox[t]{2mm}{\multirow{5}{*}{\rotatebox[origin=c]{90}{\textsc{\scriptsize VLCS}}}} 
& ERM    & 99.15 $\pm$ 0.01 & 64.43 $\pm$ 1.04 & 75.95 $\pm$ 0.40 & \textbf{81.04} $\pm$ 0.86 & \textbf{80.14} \\
& IRM    & 98.26 $\pm$ 0.21 & 64.57 $\pm$ 1.19 & 73.08 $\pm$ 3.43 & 78.20 $\pm$ 2.91 & 78.53 \\
& Mixup  & 98.83 $\pm$ 0.03 & \textbf{65.90} $\pm$ 1.40 & 75.81 $\pm$ 0.12 & 79.21 $\pm$ 2.84 & 79.94 \\
& MBDG   & \textbf{99.23} $\pm$ 0.12 & 64.10 $\pm$ 0.43 & 71.02 $\pm$ 0.70 & 77.02 $\pm$ 0.01 & 77.84 \\
\cmidrule{2-7}
& \sysname{} (ours)   & 98.37 $\pm$ 0.73 & 62.90 $\pm$ 0.50 & \textbf{76.60} $\pm$ 1.10 & 75.00 $\pm$ 3.08 & 78.22 \\
\midrule
& Methods & L100 & L38 & L43 & L46 & Avg \\
\cmidrule{2-7}
\parbox[t]{2mm}{\multirow{5}{*}{\rotatebox[origin=c]{90}{\textsc{\scriptsize TerraIncognita}}}} 
& ERM    & 44.27 $\pm$ 2.78 & \textbf{56.73} $\pm$ 5.03 & 58.64 $\pm$ 3.75 & 49.21 $\pm$ 1.13 & 52.21 $\pm$ 2.92 \\
& IRM    & 52.53 $\pm$ 9.82 & 45.04 $\pm$ 13.74 & 63.29 $\pm$ 2.24 & 47.28 $\pm$ 2.36 & 52.04 $\pm$ 3.54 \\
& Mixup  & 57.52 $\pm$ 1.86 & 53.12 $\pm$ 0.14 & \textbf{63.58} $\pm$ 0.68 & 43.56 $\pm$ 4.02 & 54.45 $\pm$ 3.67 \\
& MBDG   & 41.74 $\pm$ 7.38 & 36.87 $\pm$ 13.32 & 56.23 $\pm$ 0.94 & 41.29 $\pm$ 1.18 & 44.03 $\pm$ 3.71 \\
\cmidrule{2-7}
& \sysname{} (ours)  & \textbf{52.83} $\pm$ 4.83 & 54.67 $\pm$ 3.46 & 61.34 $\pm$ 0.45 & \textbf{50.98} $\pm$ 0.19 & \textbf{55.61} $\pm$ 0.98 \\
\bottomrule
\end{tabular}
\end{table*}

\begin{table*}[!t]
\centering
\scriptsize
\caption{\textsc{ColoredMNIST} AUROC Performance Evaluation Details. The AUROC values are the average across all trials and choices of OOD class. Top results are highlighted in \textbf{bold}.}
\begin{tabular}{c|l|c|c|c|c}
\toprule
Data & Methods & OCSVM & DDU & MSP & Energy \\ 
\midrule
\parbox[t]{2mm}{\multirow{5}{*}{\rotatebox[origin=c]{90}{+90\%}}} 
& ERM    & 53.17 $\pm$ 2.80 & 50.54 $\pm$ 5.63 & 49.72 $\pm$ 2.29 & 50.54 $\pm$ 2.74 \\
& IRM    & 53.17 $\pm$ 0.49 & 52.36 $\pm$ 2.05 & 57.20 $\pm$ 2.21 & 51.94 $\pm$ 6.06 \\
& Mixup  & 55.84 $\pm$ 1.90 & 53.20 $\pm$ 4.43 & 53.00 $\pm$ 1.74 & 49.50 $\pm$ 2.45 \\
& MBDG   & 56.72 $\pm$ 4.34 & 71.54 $\pm$ 8.99 & 62.94 $\pm$ 3.60 & 66.34 $\pm$ 4.92 \\
\cmidrule{2-6}
& \sysname{} (ours)   & \textbf{76.95} $\pm$ 2.86 & \textbf{79.61} $\pm$ 3.24 & \textbf{86.19} $\pm$ 2.13 & \textbf{86.28} $\pm$ 2.09 \\
\midrule
\parbox[t]{2mm}{\multirow{5}{*}{\rotatebox[origin=c]{90}{+80\%}}} 
& ERM    & 51.10 $\pm$ 2.17 & 48.74 $\pm$ 5.79 & 50.78 $\pm$ 1.72 & 50.38 $\pm$ 3.49 \\
& IRM    & 52.51 $\pm$ 3.03 & 48.06 $\pm$ 3.76 & 49.16 $\pm$ 1.57 & 48.87 $\pm$ 3.66 \\
& Mixup  & 52.65 $\pm$ 3.09 & 52.08 $\pm$ 3.44 & 49.50 $\pm$ 2.08 & 51.88 $\pm$ 2.27 \\
& MBDG   & 54.26 $\pm$ 4.25 & 69.70 $\pm$ 4.15 & 65.52 $\pm$ 5.91 & 64.89 $\pm$ 5.61 \\
\cmidrule{2-6}
& \sysname{} (ours)   & \textbf{70.89} $\pm$ 3.08 & \textbf{72.48} $\pm$ 5.30 & \textbf{81.58} $\pm$ 2.67 & \textbf{80.88} $\pm$ 2.46 \\
\midrule
\parbox[t]{2mm}{\multirow{5}{*}{\rotatebox[origin=c]{90}{-90\%}}} 
& ERM    & 51.11 $\pm$ 2.19 & 57.23 $\pm$ 5.34 & 46.28 $\pm$ 2.09 & 50.26 $\pm$ 3.60 \\
& IRM    & 53.28 $\pm$ 1.21 & 50.05 $\pm$ 3.54 & 46.98 $\pm$ 1.55 & 46.90 $\pm$ 2.39 \\
& Mixup  & 51.20 $\pm$ 3.66 & 51.09 $\pm$ 2.95 & 48.26 $\pm$ 1.17 & 47.55 $\pm$ 3.22 \\
& MBDG   & 51.86 $\pm$ 3.98 & 47.46 $\pm$ 6.35 & 46.93 $\pm$ 4.22 & 48.59 $\pm$ 3.11 \\
\cmidrule{2-6}
& \sysname{} (ours)   & \textbf{71.24} $\pm$ 4.96 & \textbf{72.62} $\pm$ 3.66 & \textbf{77.67} $\pm$ 1.97 & \textbf{77.53} $\pm$ 1.80 \\
\bottomrule
\end{tabular}
\label{tab:ood-details-cmnist-auroc}
\end{table*}

\begin{table*}[!t]
\centering
\scriptsize
\caption{\textsc{ColoredMNIST} AUPR Performance Evaluation Details. The AUPR values are the average across all trials and choices of OOD class. Top results are highlighted in \textbf{bold}.}
\begin{tabular}{c|l|c|c|c|c}
\toprule
Data & Methods & OCSVM & DDU & MSP & Energy \\ 
\midrule
\parbox[t]{2mm}{\multirow{5}{*}{\rotatebox[origin=c]{90}{+90\%}}} 
& ERM    & 11.47 $\pm$ 0.39 & 9.16 $\pm$ 0.89 & 9.81 $\pm$ 0.34 & 10.38 $\pm$ 0.61 \\
& IRM    & 11.27 $\pm$ 0.41 & 10.61 $\pm$ 0.82 & 12.60 $\pm$ 0.89 & 11.35 $\pm$ 1.92 \\
& Mixup  & 12.08 $\pm$ 1.10 & 9.09 $\pm$ 0.93 & 11.60 $\pm$ 0.54 & 9.70 $\pm$ 0.69 \\
& MBDG   & 16.86 $\pm$ 6.52 & 8.27 $\pm$ 1.00 & 15.11 $\pm$ 1.69 & 18.88 $\pm$ 3.88 \\
\cmidrule{2-6}
& \sysname{} (ours)   & \textbf{55.68} $\pm$ 0.39 & \textbf{40.71} $\pm$ 0.95 & \textbf{58.04} $\pm$ 0.43 & \textbf{58.05} $\pm$ 0.43 \\
\midrule
\parbox[t]{2mm}{\multirow{5}{*}{\rotatebox[origin=c]{90}{+80\%}}} 
& ERM    & 10.49 $\pm$ 0.26 & 8.94 $\pm$ 1.06 & 10.52 $\pm$ 0.50 & 10.49 $\pm$ 1.17 \\
& IRM    & 11.23 $\pm$ 1.21 & 9.08 $\pm$ 0.49 & 9.90 $\pm$ 0.44 & 9.91 $\pm$ 0.93 \\
& Mixup  & 11.23 $\pm$ 1.25 & 9.15 $\pm$ 0.51 & 10.19 $\pm$ 0.48 & 10.68 $\pm$ 0.46 \\
& MBDG   & 14.64 $\pm$ 2.39 & 7.75 $\pm$ 0.84 & 17.98 $\pm$ 3.26 & 16.40 $\pm$ 2.16 \\
\cmidrule{2-6}
& \sysname{} (ours)   & \textbf{54.82} $\pm$ 0.83 & \textbf{43.54} $\pm$ 1.81 & \textbf{57.43} $\pm$ 0.38 & \textbf{57.24} $\pm$ 0.33 \\
\midrule
\parbox[t]{2mm}{\multirow{5}{*}{\rotatebox[origin=c]{90}{-90\%}}} 
& ERM    & 10.21 $\pm$ 0.34 & 9.29 $\pm$ 0.40 & 9.17 $\pm$ 0.41 & 10.53 $\pm$ 0.96 \\
& IRM    & 10.94 $\pm$ 0.70 & 8.58 $\pm$ 0.21 & 9.06 $\pm$ 0.45 & 9.15 $\pm$ 0.42 \\
& Mixup  & 9.52 $\pm$ 0.19 & 9.02 $\pm$ 0.39 & 9.49 $\pm$ 0.17 & 9.54 $\pm$ 0.76 \\
& MBDG   & 10.91 $\pm$ 1.45 & 8.69 $\pm$ 0.83 & 9.41 $\pm$ 0.94 & 10.19 $\pm$ 0.80 \\
\cmidrule{2-6}
& \sysname{} (ours)   & \textbf{55.35} $\pm$ 0.97 & \textbf{43.15} $\pm$ 1.06 & \textbf{56.82} $\pm$ 0.35 & \textbf{56.82} $\pm$ 0.32 \\
\bottomrule
\end{tabular}
\label{tab:ood-details-cmnist-aupr}
\end{table*}

\begin{table*}[!t]
\centering
\scriptsize
\caption{\textsc{PACS} AUROC Performance Evaluation Details. The AUROC values are the average across all trials and choices of OOD class. Top results are highlighted in \textbf{bold}.}
\begin{tabular}{c|l|c|c|c|c}
\toprule
Data & Methods & OCSVM & DDU & MSP & Energy \\ 
\midrule
\parbox[t]{2mm}{\multirow{5}{*}{\rotatebox[origin=c]{90}{Art Painting}}} 
& ERM    & 50.15 $\pm$ 5.27 & 53.70 $\pm$ 7.56 & 79.79 $\pm$ 4.28 & 80.00 $\pm$ 5.81 \\
& IRM    & 58.81 $\pm$ 4.86 & 48.38 $\pm$ 12.87 & 77.08 $\pm$ 5.31 & 78.05 $\pm$ 7.22 \\
& Mixup  & 38.53 $\pm$ 3.25 & 70.06 $\pm$ 3.98 & 75.17 $\pm$ 5.46 & 75.14 $\pm$ 6.07 \\
& MBDG   & \textbf{61.09} $\pm$ 6.14 & 48.35 $\pm$ 10.66 & 75.70 $\pm$ 1.86 & 75.62 $\pm$ 4.02 \\
\cmidrule{2-6}
& \sysname{} (ours)   & 52.47 $\pm$ 7.69 & \textbf{81.15} $\pm$ 4.67 & \textbf{83.02} $\pm$ 3.52 & \textbf{84.50} $\pm$ 4.95 \\
\midrule
\parbox[t]{2mm}{\multirow{5}{*}{\rotatebox[origin=c]{90}{Cartoon}}} 
& ERM    & 44.38 $\pm$ 16.92 & 65.79 $\pm$ 14.52 & 73.83 $\pm$ 2.55 & 74.90 $\pm$ 4.06 \\
& IRM    & 45.96 $\pm$ 12.59 & 64.42 $\pm$ 7.50 & 69.06 $\pm$ 8.36 & 72.18 $\pm$ 9.50 \\
& Mixup  & 29.09 $\pm$ 7.13 & 75.01 $\pm$ 5.61 & 66.83 $\pm$ 4.79 & 64.28 $\pm$ 4.25 \\
& MBDG   & 46.63 $\pm$ 4.91 & 63.72 $\pm$ 0.68 & 68.72 $\pm$ 4.69 & 69.28 $\pm$ 5.37 \\
\cmidrule{2-6}
& \sysname{} (ours)   & \textbf{64.85} $\pm$ 9.77 & \textbf{83.59} $\pm$ 4.45 & \textbf{80.32} $\pm$ 2.57 & \textbf{84.16} $\pm$ 2.59 \\
\midrule
\parbox[t]{2mm}{\multirow{5}{*}{\rotatebox[origin=c]{90}{Photo}}} 
& ERM    & 51.73 $\pm$ 4.91 & 59.06 $\pm$ 11.86 & 81.83 $\pm$ 7.00 & 83.22 $\pm$ 6.74 \\
& IRM    & \textbf{63.61} $\pm$ 9.24 & 51.14 $\pm$ 12.63 & 92.05 $\pm$ 0.38 & 93.41 $\pm$ 0.79 \\
& Mixup  & 39.33 $\pm$ 24.24 & 64.13 $\pm$ 22.94 & 87.13 $\pm$ 1.69 & 85.21 $\pm$ 2.78 \\
& MBDG   & 46.25 $\pm$ 2.10 & 69.04 $\pm$ 7.78 & 84.67 $\pm$ 4.76 & 85.37 $\pm$ 5.06 \\
\cmidrule{2-6}
& \sysname{} (ours)   & 54.68 $\pm$ 6.24 & \textbf{93.75} $\pm$ 2.99 & \textbf{93.31} $\pm$ 2.78 & \textbf{94.87} $\pm$ 2.82 \\
\midrule
\parbox[t]{2mm}{\multirow{5}{*}{\rotatebox[origin=c]{90}{Sketch}}} 
& ERM    & 51.89 $\pm$ 4.83 & 43.82 $\pm$ 1.94 & 76.71 $\pm$ 4.48 & 82.38 $\pm$ 5.30 \\
& IRM    & 57.32 $\pm$ 1.12 & 37.98 $\pm$ 8.25 & 74.02 $\pm$ 0.59 & 80.64 $\pm$ 1.95 \\
& Mixup  & 34.22 $\pm$ 10.10 & 66.88 $\pm$ 6.33 & 69.68 $\pm$ 2.70 & 71.94 $\pm$ 0.63 \\
& MBDG   & \textbf{72.03} $\pm$ 9.26 & 34.47 $\pm$ 8.42 & 76.64 $\pm$ 2.01 & 83.76 $\pm$ 1.87 \\
\cmidrule{2-6}
& \sysname{} (ours)   & 62.82 $\pm$ 12.30 & \textbf{84.09} $\pm$ 3.71 & \textbf{82.45} $\pm$ 1.87 & \textbf{88.02} $\pm$ 2.56 \\
\bottomrule
\end{tabular}
\label{tab:ood-details-pacs-auroc}
\end{table*}

\begin{table*}[!t]
\centering
\scriptsize
\caption{\textsc{PACS} AUPR Performance Evaluation Details. The AUPR values are the average across all trials and choices of OOD class. Top results are highlighted in \textbf{bold}.}
\begin{tabular}{c|l|c|c|c|c}
\toprule
Data & Methods & OCSVM & DDU & MSP & Energy \\ 
\midrule
\parbox[t]{2mm}{\multirow{5}{*}{\rotatebox[origin=c]{90}{Art Painting}}} 
& ERM    & 20.56 $\pm$ 3.01 & 20.42 $\pm$ 8.25 & 36.27 $\pm$ 9.44 & 38.38 $\pm$ 10.66 \\
& IRM    & 24.98 $\pm$ 7.52 & 21.06 $\pm$ 5.80 & 32.80 $\pm$ 7.37 & 36.08 $\pm$ 8.47 \\
& Mixup  & 17.30 $\pm$ 6.03 & 29.87 $\pm$ 2.54 & 34.45 $\pm$ 9.65 & 36.13 $\pm$ 9.46 \\
& MBDG   & 22.77 $\pm$ 7.06 & 17.18 $\pm$ 4.19 & 28.06 $\pm$ 3.99 & 29.49 $\pm$ 4.16 \\
\cmidrule{2-6}
& \sysname{} (ours)   & \textbf{45.29} $\pm$ 1.12 & \textbf{56.06} $\pm$ 1.39 & \textbf{56.66} $\pm$ 0.96 & \textbf{56.80} $\pm$ 1.26 \\
\midrule
\parbox[t]{2mm}{\multirow{5}{*}{\rotatebox[origin=c]{90}{Cartoon}}} 
& ERM    & 19.06 $\pm$ 9.07 & 26.73 $\pm$ 9.27 & 24.95 $\pm$ 6.82 & 31.81 $\pm$ 7.08 \\
& IRM    & 19.90 $\pm$ 8.15 & 25.35 $\pm$ 1.99 & 24.59 $\pm$ 9.34 & 30.65 $\pm$ 12.64 \\
& Mixup  & 11.17 $\pm$ 4.08 & 31.59 $\pm$ 3.00 & 21.24 $\pm$ 7.01 & 20.71 $\pm$ 6.73 \\
& MBDG   & 16.45 $\pm$ 4.69 & 21.63 $\pm$ 8.58 & 25.05 $\pm$ 7.87 & 26.60 $\pm$ 9.57 \\
\cmidrule{2-6}
& \sysname{} (ours)   & \textbf{43.00} $\pm$ 2.83 & \textbf{56.84} $\pm$ 1.30 & \textbf{56.68} $\pm$ 0.83 & \textbf{57.20} $\pm$ 0.87 \\
\midrule
\parbox[t]{2mm}{\multirow{5}{*}{\rotatebox[origin=c]{90}{Photo}}} 
& ERM    & 22.07 $\pm$ 5.16 & 34.40 $\pm$ 10.62 & 40.20 $\pm$ 6.77 & 48.01 $\pm$ 7.05 \\
& IRM    & 32.43 $\pm$ 6.58 & 29.75 $\pm$ 11.95 & 56.93 $\pm$ 6.41 & \textbf{64.63} $\pm$ 8.54 \\
& Mixup  & 32.07 $\pm$ 18.91 & 40.81 $\pm$ 21.82 & 51.14 $\pm$ 7.20 & 54.33 $\pm$ 8.06 \\
& MBDG   & 24.21 $\pm$ 3.66 & 37.28 $\pm$ 5.35 & 44.74 $\pm$ 5.32 & 47.32 $\pm$ 5.65 \\
\cmidrule{2-6}
& \sysname{} (ours)   & \textbf{42.29} $\pm$ 3.89 & \textbf{58.90} $\pm$ 0.41 & \textbf{58.79} $\pm$ 0.40 & 59.08 $\pm$ 0.43 \\
\midrule
\parbox[t]{2mm}{\multirow{5}{*}{\rotatebox[origin=c]{90}{Sketch}}} 
& ERM    & 17.80 $\pm$ 7.22 & 18.68 $\pm$ 9.44 & 29.13 $\pm$ 11.64 & 37.62 $\pm$ 14.14 \\
& IRM    & 18.05 $\pm$ 5.48 & 12.95 $\pm$ 6.27 & 26.47 $\pm$ 8.48 & 37.21 $\pm$ 9.96 \\
& Mixup  & 9.70 $\pm$ 2.19 & 31.91 $\pm$ 13.65 & 23.98 $\pm$ 7.93 & 29.70 $\pm$ 10.09 \\
& MBDG   & 24.68 $\pm$ 7.68 & 13.46 $\pm$ 6.68 & 29.86 $\pm$ 8.27 & 41.97 $\pm$ 9.78 \\
\cmidrule{2-6}
& \sysname{} (ours)   & \textbf{42.89} $\pm$ 7.65 & \textbf{57.40} $\pm$ 1.13 & \textbf{56.92} $\pm$ 1.33 & \textbf{57.74} $\pm$ 1.19 \\
\bottomrule
\end{tabular}
\label{tab:ood-details-pacs-aupr}
\end{table*}

\begin{table*}[!t]
\centering
\scriptsize
\caption{\textsc{VLCS} AUROC Performance Evaluation Details. The AUROC values are the average across all trials and choices of OOD class. Top results are highlighted in \textbf{bold}.}
\begin{tabular}{c|l|c|c|c|c}
\toprule
Data & Methods & OCSVM & DDU & MSP & Energy \\ 
\midrule
\parbox[t]{2mm}{\multirow{5}{*}{\rotatebox[origin=c]{90}{Caltech101}}} 
& ERM    & 19.34 $\pm$ 12.10 & 82.13 $\pm$ 9.01 & 92.01 $\pm$ 4.20 & 93.62 $\pm$ 3.00 \\
& IRM    & 16.26 $\pm$ 9.22 & 80.53 $\pm$ 7.60 & 89.45 $\pm$ 7.11 & 90.44 $\pm$ 6.40 \\
& Mixup  & 14.62 $\pm$ 0.56 & 81.26 $\pm$ 7.79 & 89.60 $\pm$ 1.34 & 90.02 $\pm$ 0.37 \\
& MBDG   & 75.58 $\pm$ 1.30 & 61.02 $\pm$ 3.56 & 83.00 $\pm$ 6.66 & 87.46 $\pm$ 5.02 \\
\cmidrule{2-6}
& \sysname{} (ours)   & \textbf{90.00} $\pm$ 3.83 & \textbf{95.62} $\pm$ 2.63 & \textbf{93.34} $\pm$ 4.39 & \textbf{94.54} $\pm$ 2.88 \\
\midrule
\parbox[t]{2mm}{\multirow{5}{*}{\rotatebox[origin=c]{90}{LabelMe}}} 
& ERM    & 46.96 $\pm$ 17.42 & 37.30 $\pm$ 8.34 & 71.49 $\pm$ 3.75 & 73.24 $\pm$ 2.62 \\
& IRM    & 45.38 $\pm$ 9.26 & 37.68 $\pm$ 5.26 & 71.82 $\pm$ 3.68 & 73.63 $\pm$ 4.31 \\
& Mixup  & 28.06 $\pm$ 14.97 & 52.88 $\pm$ 20.02 & 66.82 $\pm$ 10.78 & 67.34 $\pm$ 12.70 \\
& MBDG   & 58.48 $\pm$ 14.13 & 41.32 $\pm$ 8.79 & 71.17 $\pm$ 5.37 & 74.20 $\pm$ 4.82 \\
\cmidrule{2-6}
& \sysname{} (ours)   & \textbf{61.20} $\pm$ 4.89 & \textbf{84.30} $\pm$ 9.95 & \textbf{80.52} $\pm$ 8.14 & \textbf{83.28} $\pm$ 10.02 \\
\midrule
\parbox[t]{2mm}{\multirow{5}{*}{\rotatebox[origin=c]{90}{Sun09}}} 
& ERM    & 33.54 $\pm$ 2.38 & 60.26 $\pm$ 1.68 & 54.97 $\pm$ 1.75 & 57.48 $\pm$ 1.95 \\
& IRM    & 32.98 $\pm$ 8.14 & 62.62 $\pm$ 6.77 & 56.53 $\pm$ 3.57 & 62.58 $\pm$ 0.62 \\
& Mixup  & 29.39 $\pm$ 6.23 & 63.42 $\pm$ 6.52 & 53.60 $\pm$ 6.39 & 57.02 $\pm$ 3.86 \\
& MBDG   & 62.94 $\pm$ 1.90 & 54.96 $\pm$ 3.64 & 56.04 $\pm$ 11.12 & 65.11 $\pm$ 6.70 \\
\cmidrule{2-6}
& \sysname{} (ours)   & \textbf{69.59} $\pm$ 4.00 & \textbf{76.12} $\pm$ 5.20 & \textbf{62.98} $\pm$ 1.61 & \textbf{69.56} $\pm$ 1.90 \\
\midrule
\parbox[t]{2mm}{\multirow{5}{*}{\rotatebox[origin=c]{90}{VOC2007}}} 
& ERM    & 42.00 $\pm$ 23.96 & 52.46 $\pm$ 22.50 & 59.72 $\pm$ 8.13 & 63.81 $\pm$ 3.74 \\
& IRM    & 46.15 $\pm$ 23.57 & 47.04 $\pm$ 22.12 & 58.68 $\pm$ 7.69 & 63.52 $\pm$ 8.60 \\
& Mixup  & 49.03 $\pm$ 26.46 & 41.92 $\pm$ 22.15 & 50.78 $\pm$ 1.10 & 58.34 $\pm$ 1.19 \\
& MBDG   & \textbf{54.12} $\pm$ 26.16 & 47.40 $\pm$ 4.91 & 52.18 $\pm$ 3.28 & 60.78 $\pm$ 5.91 \\
\cmidrule{2-6}
& \sysname{} (ours)   & 52.22 $\pm$ 15.13 & \textbf{64.50} $\pm$ 16.30 & \textbf{63.33} $\pm$ 2.29 & \textbf{67.16} $\pm$ 1.57 \\
\bottomrule
\end{tabular}
\label{tab:ood-details-vlcs-auroc}
\end{table*}

\begin{table*}[!t]
\centering
\scriptsize
\caption{\textsc{VLCS} AUPR Performance Evaluation Details. The AUPR values are the average across all trials and choices of OOD class. Top results are highlighted in \textbf{bold}.}
\begin{tabular}{c|l|c|c|c|c}
\toprule
Data & Methods & OCSVM & DDU & MSP & Energy \\ 
\midrule
\parbox[t]{2mm}{\multirow{5}{*}{\rotatebox[origin=c]{90}{Caltech101}}} 
& ERM    & 5.96 $\pm$ 0.32 & 41.22 $\pm$ 27.30 & 59.23 $\pm$ 5.75 & 64.01 $\pm$ 6.39 \\
& IRM    & 7.41 $\pm$ 2.06 & 43.18 $\pm$ 29.56 & 57.72 $\pm$ 0.39 & 63.62 $\pm$ 1.44 \\
& Mixup  & 7.47 $\pm$ 2.57 & 36.34 $\pm$ 20.21 & 53.30 $\pm$ 21.92 & 57.57 $\pm$ 17.11 \\
& MBDG   & 4.45 $\pm$ 0.45 & 17.92 $\pm$ 5.22 & 30.86 $\pm$ 15.82 & 42.27 $\pm$ 20.23 \\
\cmidrule{2-6}
& \sysname{} (ours)   & \textbf{58.19} $\pm$ 0.60 & \textbf{69.40} $\pm$ 0.44 & \textbf{69.36} $\pm$ 0.43 & \textbf{69.46} $\pm$ 0.28 \\
\midrule
\parbox[t]{2mm}{\multirow{5}{*}{\rotatebox[origin=c]{90}{LabelMe}}} 
& ERM    & 4.04 $\pm$ 2.38 & 4.38 $\pm$ 1.80 & 5.92 $\pm$ 0.58 & 9.27 $\pm$ 0.01 \\
& IRM    & 4.18 $\pm$ 1.18 & 5.68 $\pm$ 0.74 & 6.22 $\pm$ 0.62 & 7.94 $\pm$ 1.69 \\
& Mixup  & 3.86 $\pm$ 2.12 & 31.93 $\pm$ 25.01 & 7.12 $\pm$ 2.56 & 13.54 $\pm$ 8.80 \\
& MBDG   & 3.62 $\pm$ 0.80 & 20.69 $\pm$ 15.79 & 6.49 $\pm$ 0.35 & 7.99 $\pm$ 1.81 \\
\cmidrule{2-6}
& \sysname{} (ours)   & \textbf{42.01} $\pm$ 5.57 & \textbf{49.06} $\pm$ 0.54 & \textbf{48.94} $\pm$ 0.34 & \textbf{48.96} $\pm$ 0.60 \\
\midrule
\parbox[t]{2mm}{\multirow{5}{*}{\rotatebox[origin=c]{90}{Sun09}}} 
& ERM    & 13.12 $\pm$ 12.66 & 19.10 $\pm$ 17.76 & 16.81 $\pm$ 16.07 & 19.82 $\pm$ 19.06 \\
& IRM    & 13.94 $\pm$ 13.52 & 19.39 $\pm$ 16.71 & 16.18 $\pm$ 15.22 & 21.50 $\pm$ 20.22 \\
& Mixup  & 12.56 $\pm$ 12.16 & 22.20 $\pm$ 15.46 & 15.00 $\pm$ 13.98 & 19.04 $\pm$ 14.78 \\
& MBDG   & 13.66 $\pm$ 13.20 & 19.48 $\pm$ 17.74 & 14.42 $\pm$ 13.16 & 19.44 $\pm$ 18.00 \\
\cmidrule{2-6}
& \sysname{} (ours)   & \textbf{19.04} $\pm$ 19.64 & \textbf{33.08} $\pm$ 6.76 & \textbf{28.56} $\pm$ 11.04 & \textbf{30.20} $\pm$ 9.43 \\
\midrule
\parbox[t]{2mm}{\multirow{5}{*}{\rotatebox[origin=c]{90}{VOC2007}}} 
& ERM    & 12.14 $\pm$ 6.24 & 21.12 $\pm$ 12.25 & 16.14 $\pm$ 6.21 & 17.41 $\pm$ 3.77 \\
& IRM    & 13.24 $\pm$ 7.20 & 14.74 $\pm$ 6.41 & 14.80 $\pm$ 3.46 & 18.22 $\pm$ 5.58 \\
& Mixup  & 17.34 $\pm$ 11.00 & 16.04 $\pm$ 8.77 & 11.00 $\pm$ 0.22 & 14.40 $\pm$ 0.41 \\
& MBDG   & 11.63 $\pm$ 5.67 & 16.54 $\pm$ 7.87 & 11.92 $\pm$ 1.01 & 14.92 $\pm$ 0.98 \\
\cmidrule{2-6}
& \sysname{} (ours)   & \textbf{28.42} $\pm$ 3.71 & \textbf{33.38} $\pm$ 3.63 & \textbf{32.76} $\pm$ 0.20 & \textbf{33.55} $\pm$ 0.39 \\
\bottomrule
\end{tabular}
\label{tab:ood-details-vlcs-aupr}
\end{table*}

\begin{table*}[!t]
\centering
\scriptsize
\caption{\textsc{TerraIncognita} AUROC Performance Evaluation Details. The AUROC values are the average across all trials and choices of OOD class. Top results are highlighted in \textbf{bold}.}
\begin{tabular}{c|l|c|c|c|c}
\toprule
Data & Methods & OCSVM & DDU & MSP & Energy \\ 
\midrule
\parbox[t]{2mm}{\multirow{5}{*}{\rotatebox[origin=c]{90}{L100}}} 
& ERM    & 36.53 $\pm$ 10.87 & 49.70 $\pm$ 16.20 & 56.36 $\pm$ 12.78 & 57.44 $\pm$ 20.36 \\
& IRM    & 37.02 $\pm$ 16.40 & 54.02 $\pm$ 1.95 & 57.28 $\pm$ 23.99 & 60.78 $\pm$ 25.82 \\
& Mixup  & 48.94 $\pm$ 22.70 & 55.33 $\pm$ 10.78 & 67.18 $\pm$ 15.34 & 69.24 $\pm$ 21.06 \\
& MBDG   & 44.93 $\pm$ 3.00 & 49.07 $\pm$ 19.80 & 47.58 $\pm$ 8.01 & 54.44 $\pm$ 20.26 \\
\cmidrule{2-6}
& \sysname{} (ours)   & \textbf{51.08} $\pm$ 5.66 & \textbf{63.25} $\pm$ 6.69 & \textbf{69.39} $\pm$ 9.76 & \textbf{71.46} $\pm$ 17.34 \\
\midrule
\parbox[t]{2mm}{\multirow{5}{*}{\rotatebox[origin=c]{90}{L38}}} 
& ERM    & 44.82 $\pm$ 4.18 & 44.06 $\pm$ 1.54 & 50.28 $\pm$ 2.20 & 53.30 $\pm$ 9.32 \\
& IRM    & 41.07 $\pm$ 3.10 & 52.68 $\pm$ 7.95 & 60.22 $\pm$ 2.92 & 64.00 $\pm$ 10.07 \\
& Mixup  & 38.54 $\pm$ 8.26 & 59.72 $\pm$ 1.62 & 56.52 $\pm$ 9.63 & 57.36 $\pm$ 16.49 \\
& MBDG   & 45.12 $\pm$ 9.61 & 59.83 $\pm$ 3.54 & 58.98 $\pm$ 15.14 & 56.22 $\pm$ 18.94 \\
\cmidrule{2-6}
& \sysname{} (ours)   & \textbf{51.24} $\pm$ 0.51 & \textbf{61.77} $\pm$ 2.34 & \textbf{71.62} $\pm$ 7.85 & \textbf{70.16} $\pm$ 12.56 \\
\midrule
\parbox[t]{2mm}{\multirow{5}{*}{\rotatebox[origin=c]{90}{L43}}} 
& ERM    & 50.50 $\pm$ 5.34 & 45.76 $\pm$ 1.59 & 49.31 $\pm$ 5.93 & 56.56 $\pm$ 2.07 \\
& IRM    & \textbf{54.34} $\pm$ 6.44 & 53.54 $\pm$ 3.67 & 53.11 $\pm$ 1.43 & 50.78 $\pm$ 8.50 \\
& Mixup  & 50.00 $\pm$ 3.39 & 57.86 $\pm$ 4.59 & 57.66 $\pm$ 1.86 & 48.97 $\pm$ 8.17 \\
& MBDG   & 51.11 $\pm$ 11.09 & 56.72 $\pm$ 7.30 & 52.71 $\pm$ 4.23 & 58.58 $\pm$ 1.60 \\
\cmidrule{2-6}
& \sysname{} (ours)   & 48.29 $\pm$ 5.01 & \textbf{61.10} $\pm$ 4.66 & \textbf{60.06} $\pm$ 2.38 & \textbf{62.72} $\pm$ 4.47 \\
\midrule
\parbox[t]{2mm}{\multirow{5}{*}{\rotatebox[origin=c]{90}{L46}}} 
& ERM    & 44.92 $\pm$ 13.65 & 50.04 $\pm$ 2.18 & 57.69 $\pm$ 0.31 & 61.72 $\pm$ 1.55 \\
& IRM    & 41.97 $\pm$ 10.10 & 58.07 $\pm$ 6.83 & 61.51 $\pm$ 3.57 & 66.43 $\pm$ 4.30 \\
& Mixup  & 39.82 $\pm$ 7.78 & 57.35 $\pm$ 4.79 & 57.52 $\pm$ 0.66 & 57.94 $\pm$ 5.72 \\
& MBDG   & 36.36 $\pm$ 5.03 & \textbf{59.86} $\pm$ 2.86 & 53.97 $\pm$ 6.95 & 59.08 $\pm$ 9.97 \\
\cmidrule{2-6}
& \sysname{} (ours)   & \textbf{47.06} $\pm$ 11.86 & 57.14 $\pm$ 1.14 & \textbf{69.07} $\pm$ 3.59 & \textbf{72.18} $\pm$ 0.88 \\
\bottomrule
\end{tabular}
\label{tab:ood-details-terra-auroc}
\end{table*}

\begin{table*}[!t]
\centering
\scriptsize
\caption{\textsc{TerraIncognita} AUPR Performance Evaluation Details. The AUPR values are the average across all trials and choices of OOD class. Top results are highlighted in \textbf{bold}.}
\begin{tabular}{c|l|c|c|c|c}
\toprule
Data & Methods & OCSVM & DDU & MSP & Energy \\ 
\midrule
\parbox[t]{2mm}{\multirow{5}{*}{\rotatebox[origin=c]{90}{L100}}} 
& ERM    & 14.72 $\pm$ 12.32 & 26.98 $\pm$ 25.37 & 20.55 $\pm$ 14.95 & 19.63 $\pm$ 11.00 \\
& IRM    & 28.28 $\pm$ 29.02 & 27.62 $\pm$ 26.8 & 27.56 $\pm$ 14.20 & 26.14 $\pm$ 16.14 \\
& Mixup  & \textbf{33.17} $\pm$ 33.82 & 23.98 $\pm$ 22.01 & \textbf{35.27} $\pm$ 15.09 & \textbf{31.94} $\pm$ 15.48 \\
& MBDG   & 25.56 $\pm$ 23.93 & \textbf{34.28} $\pm$ 32.96 & 24.06 $\pm$ 21.17 & 24.63 $\pm$ 17.71 \\
\cmidrule{2-6}
& \sysname{} (ours)   & 26.09 $\pm$ 23.52 & 28.86 $\pm$ 24.85 & 31.72 $\pm$ 26.00 & 31.58 $\pm$ 20.34 \\
\midrule
\parbox[t]{2mm}{\multirow{5}{*}{\rotatebox[origin=c]{90}{L38}}} 
& ERM    & 8.32 $\pm$ 6.14 & 8.36 $\pm$ 5.99 & 9.54 $\pm$ 7.48 & 13.81 $\pm$ 11.92 \\
& IRM    & 4.86 $\pm$ 5.04 & 7.20 $\pm$ 6.47 & 12.50 $\pm$ 12.16 & 19.38 $\pm$ 19.22 \\
& Mixup  & 5.66 $\pm$ 6.31 & 7.66 $\pm$ 6.82 & 13.35 $\pm$ 13.56 & 15.15 $\pm$ 15.52 \\
& MBDG   & 6.62 $\pm$ 4.24 & \textbf{12.51} $\pm$ 10.42 & 17.70 $\pm$ 16.02 & 14.33 $\pm$ 12.84 \\
\cmidrule{2-6}
& \sysname{} (ours)   & \textbf{9.67} $\pm$ 7.68 & 10.24 $\pm$ 7.90 & \textbf{18.76} $\pm$ 16.14 & \textbf{20.67} $\pm$ 18.54 \\
\midrule
\parbox[t]{2mm}{\multirow{5}{*}{\rotatebox[origin=c]{90}{L43}}} 
& ERM    & \textbf{8.50} $\pm$ 6.65 & 7.18 $\pm$ 4.84 & \textbf{9.34} $\pm$ 7.62 & \textbf{9.97} $\pm$ 7.39 \\
& IRM    & 7.91 $\pm$ 8.23 & 6.54 $\pm$ 6.25 & 5.06 $\pm$ 5.00 & 4.08 $\pm$ 3.56 \\
& Mixup  & 4.66 $\pm$ 5.08 & 5.62 $\pm$ 4.39 & 6.25 $\pm$ 4.50 & 4.40 $\pm$ 2.68 \\
& MBDG   & 7.85 $\pm$ 6.28 & 6.64 $\pm$ 3.80 & 6.10 $\pm$ 4.12 & 7.92 $\pm$ 4.76 \\
\cmidrule{2-6}
& \sysname{} (ours)   & 6.52 $\pm$ 5.10 & \textbf{8.04} $\pm$ 4.16 & 7.41 $\pm$ 5.14 & 8.01 $\pm$ 4.52 \\
\midrule
\parbox[t]{2mm}{\multirow{5}{*}{\rotatebox[origin=c]{90}{L46}}} 
& ERM    & \textbf{18.69} $\pm$ 2.80 & 26.78 $\pm$ 16.13 & 27.08 $\pm$ 12.92 & 30.30 $\pm$ 14.81 \\
& IRM    & 14.82 $\pm$ 3.83 & \textbf{30.46} $\pm$ 21.78 & 28.96 $\pm$ 15.26 & \textbf{34.61} $\pm$ 18.95 \\
& Mixup  & 12.84 $\pm$ 5.20 & 26.7 $\pm$ 18.07 & 22.01 $\pm$ 6.96 & 20.70 $\pm$ 3.84 \\
& MBDG   & 13.66 $\pm$ 5.53 & 27.38 $\pm$ 15.98 & 18.33 $\pm$ 5.35 & 21.40 $\pm$ 3.76 \\
\cmidrule{2-6}
& \sysname{} (ours)   & 18.02 $\pm$ 2.09 & 21.46 $\pm$ 9.75 & \textbf{30.06} $\pm$ 9.39 & 34.56 $\pm$ 9.04 \\
\bottomrule
\end{tabular}
\label{tab:ood-details-terra-aupr}
\end{table*}

\subsection{Domain and OOD Augmentation Mechanism}
The transformation model, $G$, plays a pivotal role in converting data from a given training domain into a synthetic one. This process involves a stochastic mechanism where the original variational vector of the input, $\mathbf{v}^e$, is substituted with a novel variational vector, $\mathbf{v}^{e'}$, which is randomly drawn from a standard normal distribution, denoted as $\mathcal{N}(0,\mathbf{I})$. Illustrative examples of these transformations are showcased in Figure~\ref{fig:styles}, revealing that $G$ can significantly alter the image domain when the target domain is known. In contrast, transformations appear more subtle in the absence of a specified target domain. Nonetheless, empirical evidence suggests that such transformations into synthetic domains are adequately effective for the acquisition of domain-invariant semantic knowledge.

As shown in Figure~\ref{fig:augmentation-mechanism}, the domain augmentation addresses the challenge of relying exclusively on ID data, which can lead to significant false positive regions due to inherent data limitations. By incorporating synthetic domain images, the model gains a more refined understanding of domain-invariant semantics, effectively minimizing the occurrence of false positives. This enhancement allows for a more accurate and reliable detection of true semantic features that are consistent across various domains, thus improving the model's overall performance.

On the other hand, the OOD augmentation utilizes Gaussian Discriminant Analysis (GDA) with specific Gaussian components for each class to scrutinize the semantic density of instances created through a semantic mixup process. This method ensures that only instances located in low-density regions are considered valid pseudo-OODs, effectively filtering out higher-density instances that do not meet the criteria for OOD. This selective retention of low-density pseudo-OODs enhances the model's ability to distinguish between true ID instances and potential out-of-distribution threats, thereby refining the OOD detection process.

\begin{figure*}[!t]
\centering
\begin{subfigure}{0.48\linewidth}
  \centering
  \includegraphics[width=\linewidth]{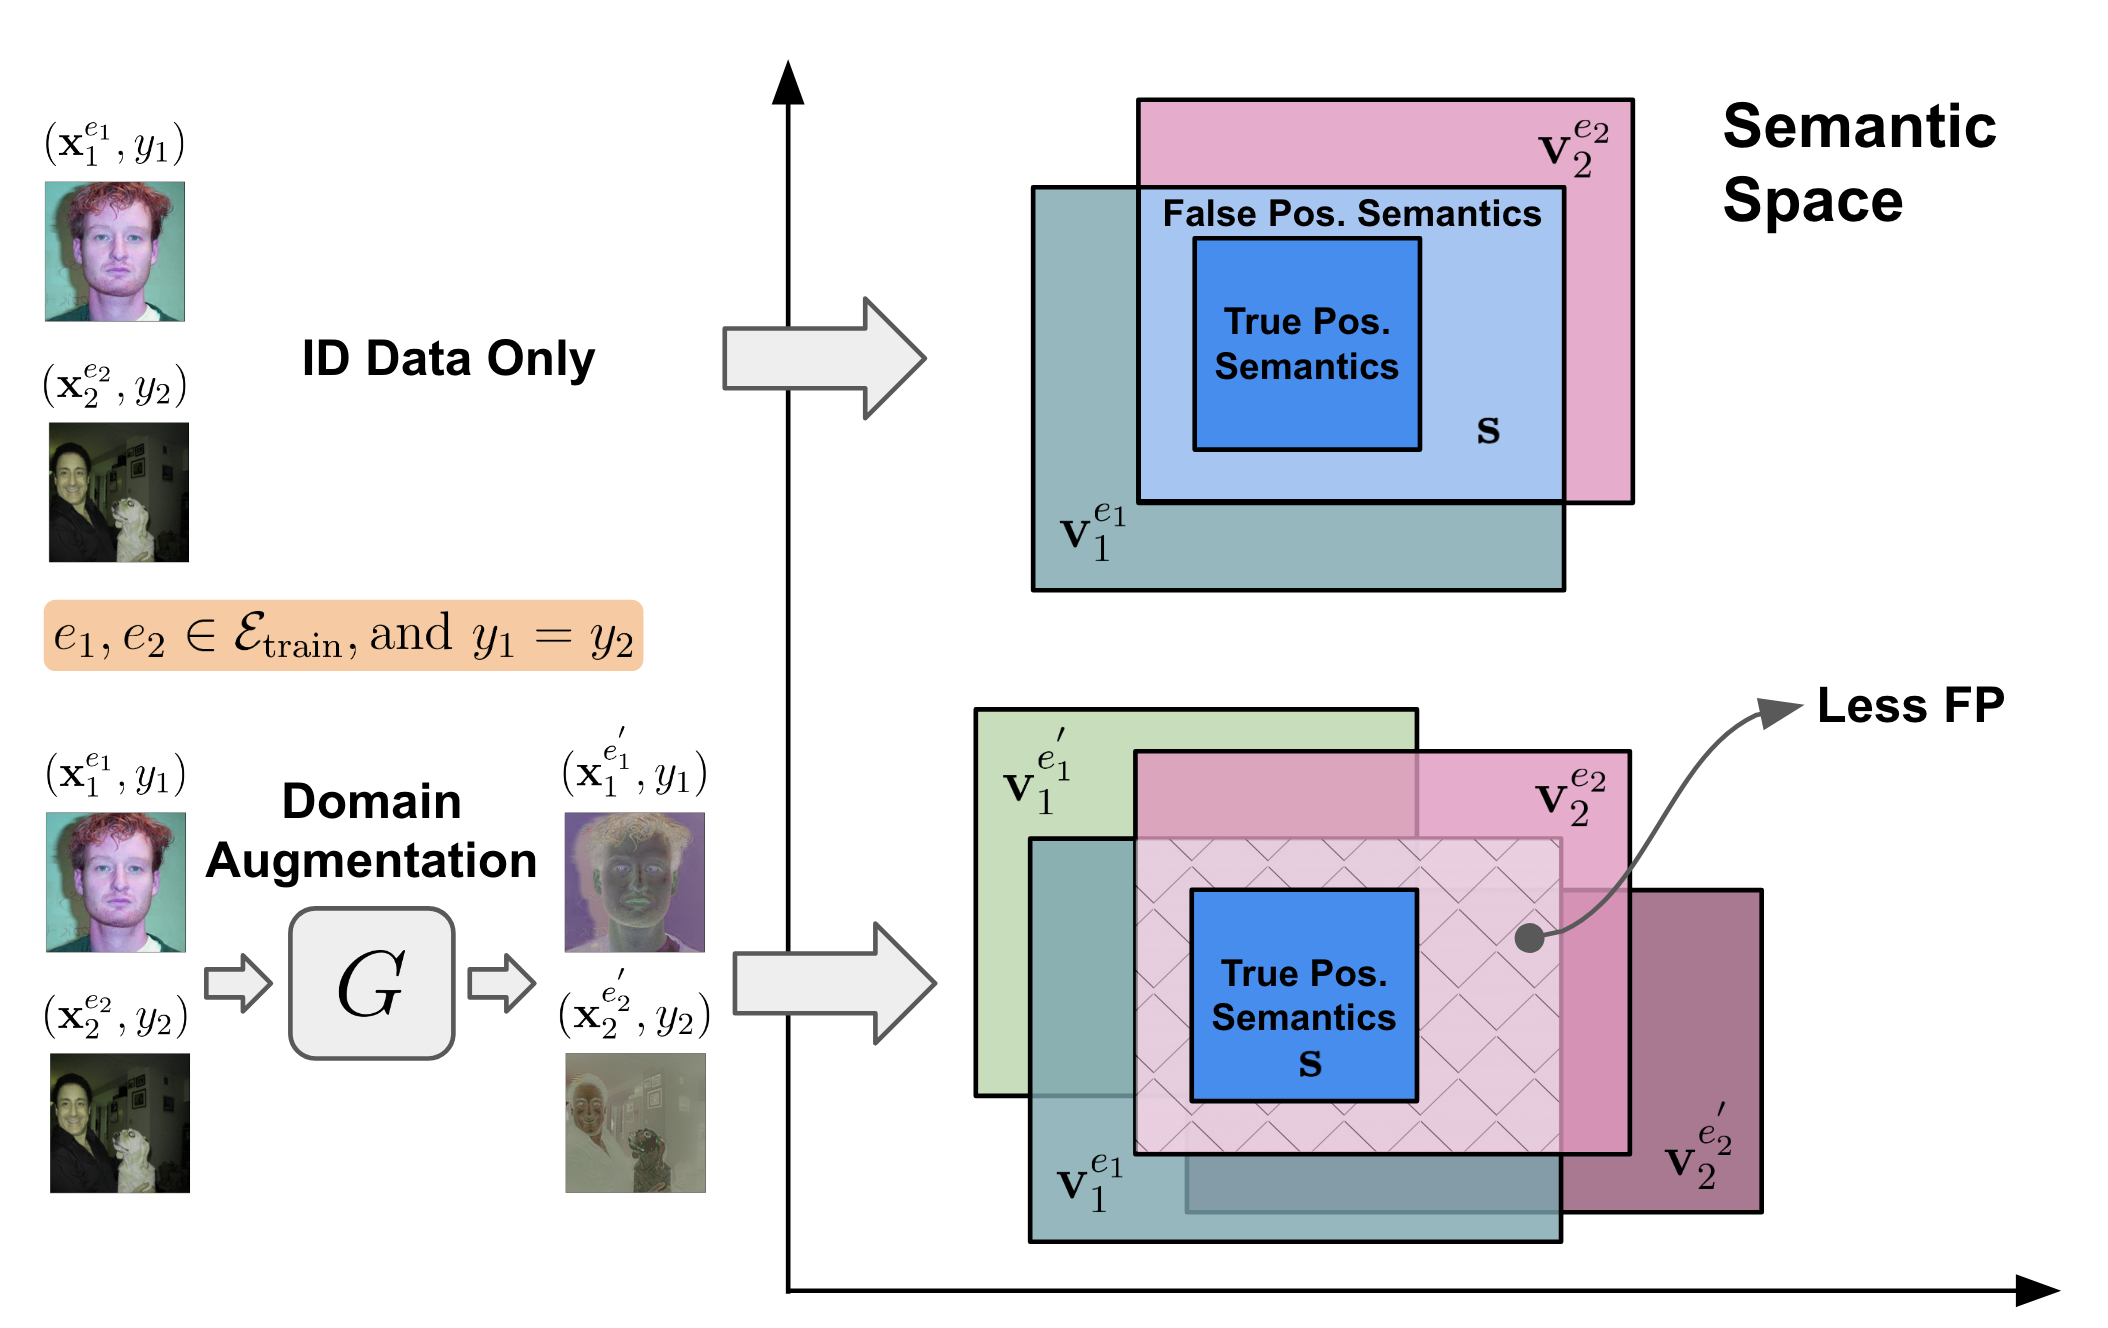}
  % \caption{Domain Augmentation Mechanism: Relying solely on ID data may result in large false positive regions due to data constraints. Employing synthetic domain images enables the model to more precisely capture domain-invariant semantics, thereby reducing the false positives.}
  \label{fig:RDG-rationale}
\end{subfigure}%
% \hfill % This will add horizontal space between the two subfigures, pushing the second to the right
\begin{subfigure}{0.48\linewidth}
  \centering
  \includegraphics[width=\linewidth]{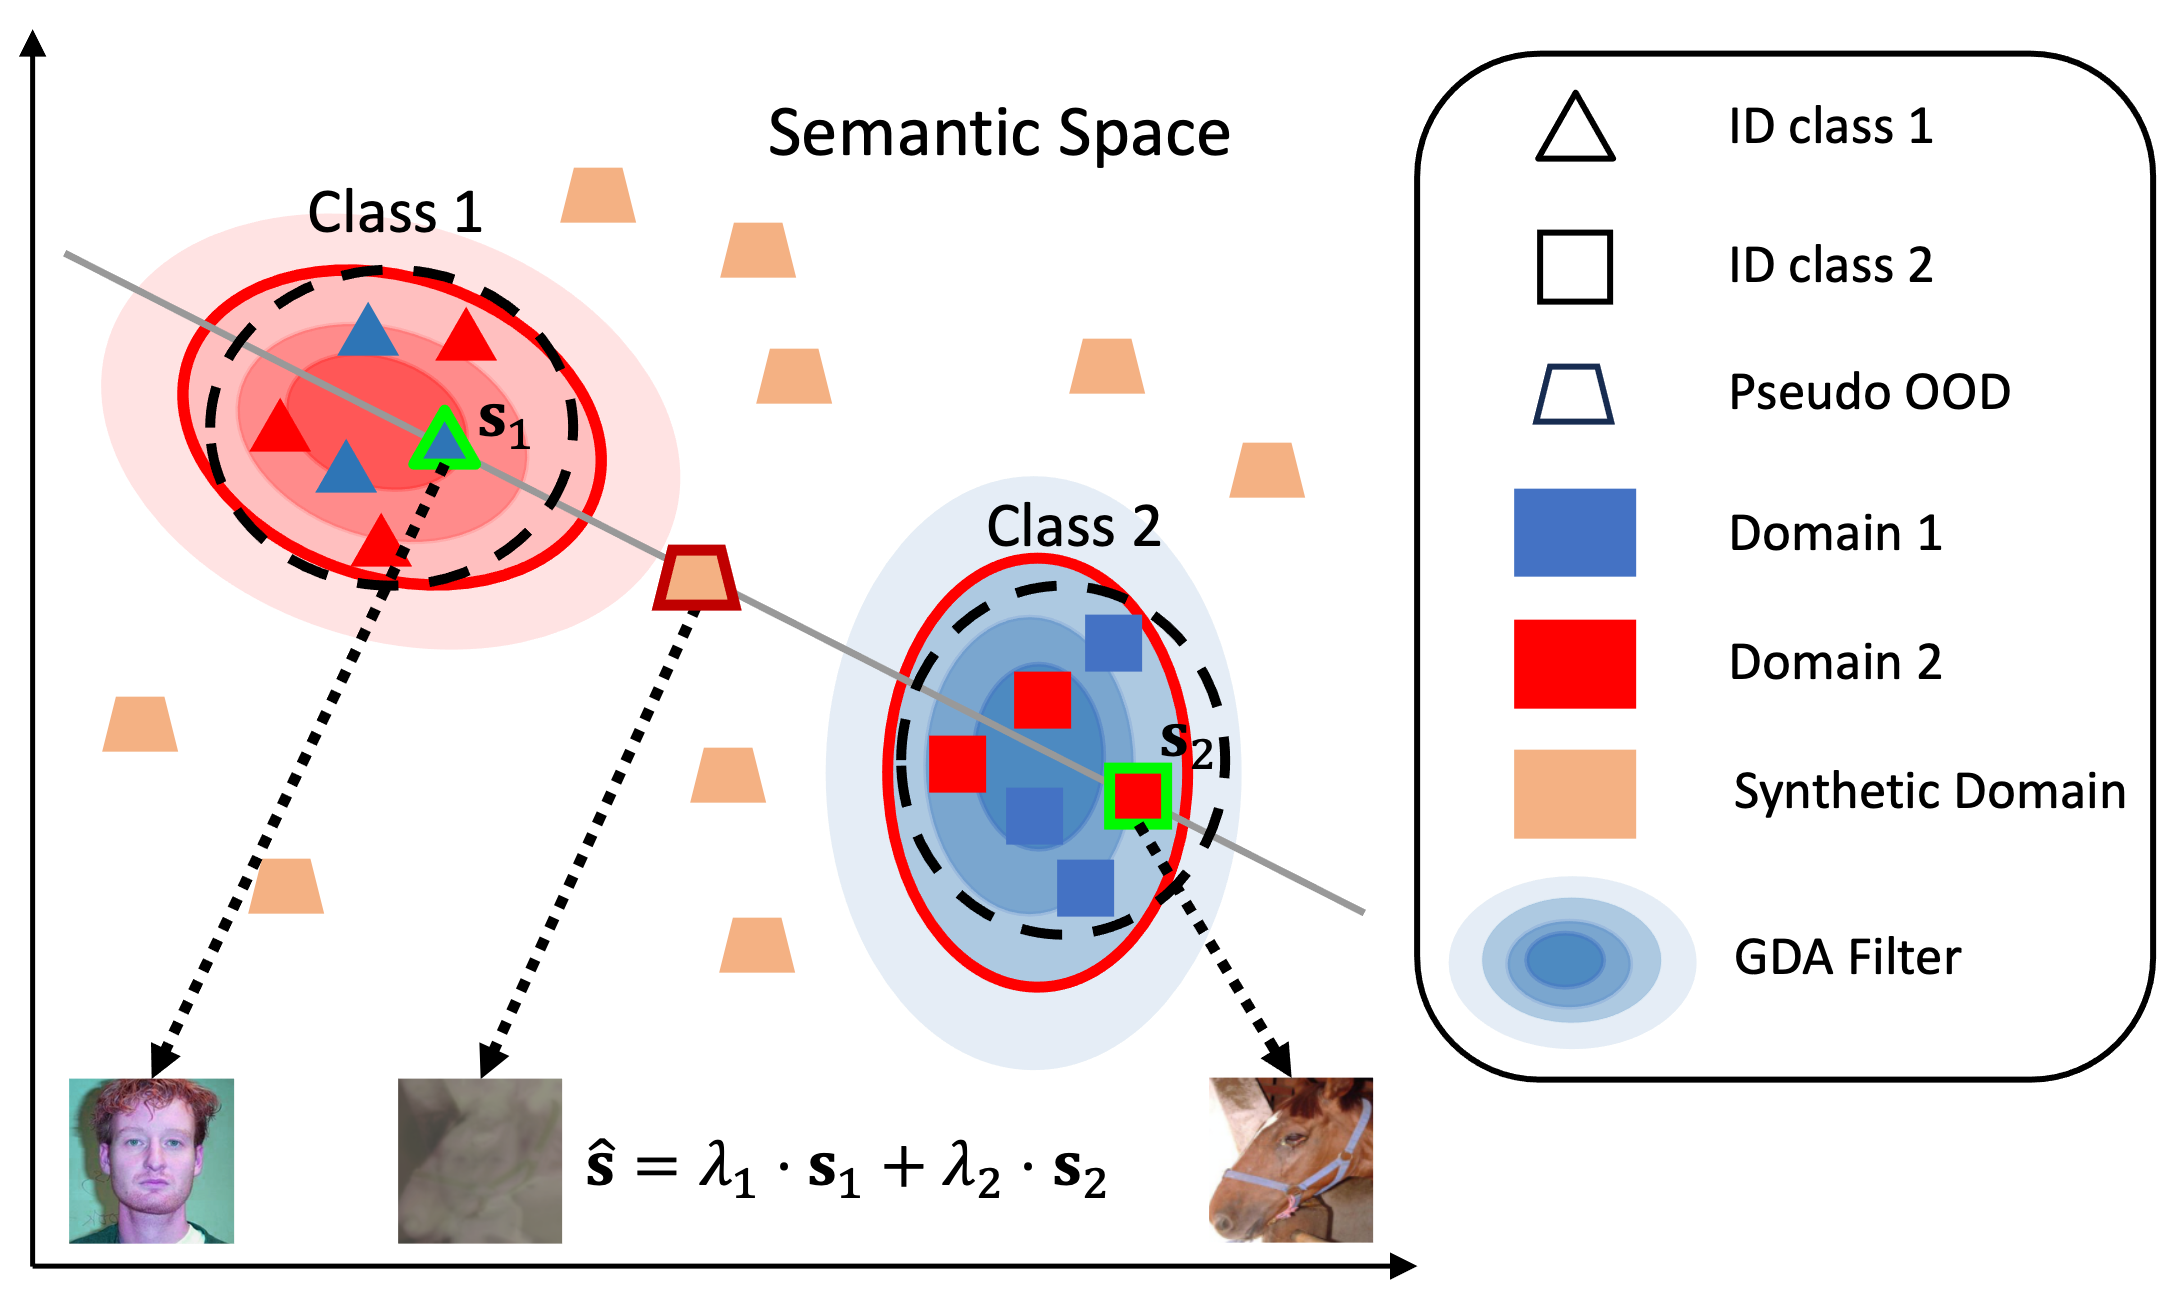}
  % \caption{OOD Augmentation Mechanism: The GDA, equipped with per-class Gaussian components, assesses the density of semantics augmented via semantic mixup, retaining only low-density instances as qualified pseudo-OODs and filtering out the rest.}
  \label{fig:GDA-filter}
\end{subfigure}
% \caption{Mechanisms of domain and OOD augmentation: Enhancing domain-invariant semantic learning and generating qualified pseudo-OODs.}
\caption{(a) Domain Augmentation Mechanism: Relying solely on ID data may result in large false positive regions due to data constraints. Employing synthetic domain images enables the model to more precisely capture domain-invariant semantics, thereby reducing the false positives. (b) OOD Augmentation Mechanism: The GDA, equipped with per-class Gaussian components, assesses the density of semantics augmented via semantic mixup, retaining only low-density instances as qualified pseudo-OODs and filtering out the rest.}
\label{fig:augmentation-mechanism}
\end{figure*}

\subsection{Feature Space Regularization versus Output Space Regularization}
\label{sec:feature_reg_vs_output_reg}

In this paper, the semantic $G$-invariance is learned through feature space regularization. Specifically, we employ the semantic $G$-invariance regularization term $R_{\text{SGI}}$ to enforce the semantic between $(\mathbf{x}^{e},y)$ and the random domain counterpart $(\mathbf{x}^{e'},y)$ in the feature space. One might wonder why we prioritize the feature space over the output space for learning semantic $G$-invariance. The primary reason is that the feature space representations contain richer information than the final outputs. As highlighted by recent neural network interpretation studies \cite{zhou2018interpreting,rauker2023toward}, deeper layers in a neural network tend to capture increasingly complex concepts. As for the output space, constrained by its feature dimension, typically represents high-level conceptual semantics, thereby limiting its representational capacity. Furthermore, OOD can take many forms, each with unique characteristics. Some OODs might exhibit only subtle deviations from the ID data. To identify such nuanced differences, it becomes imperative to leverage features with higher representational capacity.

To provide a comparative perspective, we compare \sysname{}, which employs feature space regularization, against a model where the $R_{\text{SGI}}$ term is substituted with output space regularization. Their respective t-SNE visualizations, derived from the PACS dataset with "Art Painting" as the test domain and class 6 as OODs, are presented in Figure~\ref{fig:reg-compare}. The visualization clearly demonstrates that feature space regularization yields more distinct boundaries between each class cluster. Notably, the OOD samples (represented as pink points) mostly lie in the middle with less overlapping with ID clusters. This IDicates that feature-space regularization enables \sysname{} to produce higher-quality features, enhancing the separability of OODs from IDs for downstream OOD detectors.

\begin{figure*}[!t]
\centering
    \begin{subfigure}[b]{0.5\linewidth}
       \includegraphics[width=\linewidth]{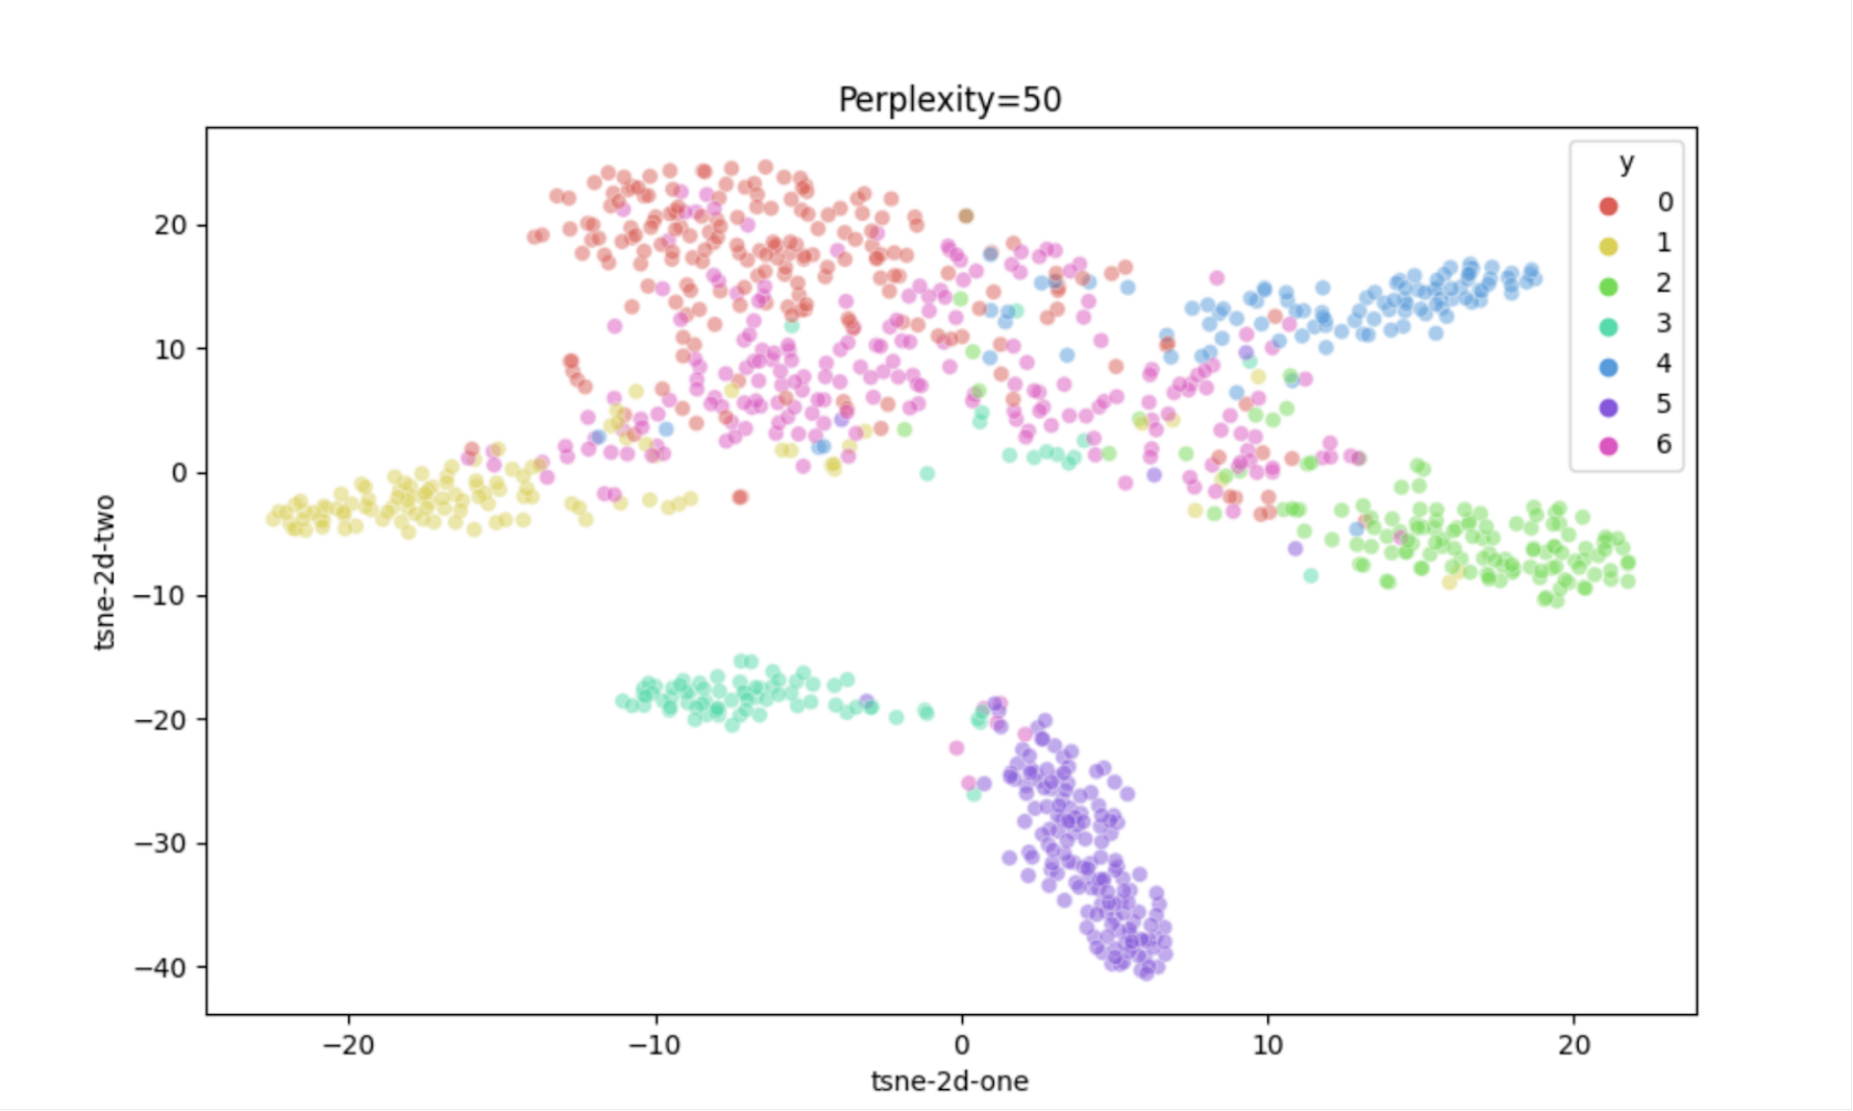}
       \caption{Output space regularization}
       \label{fig:Ng1} 
    \end{subfigure}%
    \begin{subfigure}[b]{0.5\linewidth}
       \includegraphics[width=\linewidth]{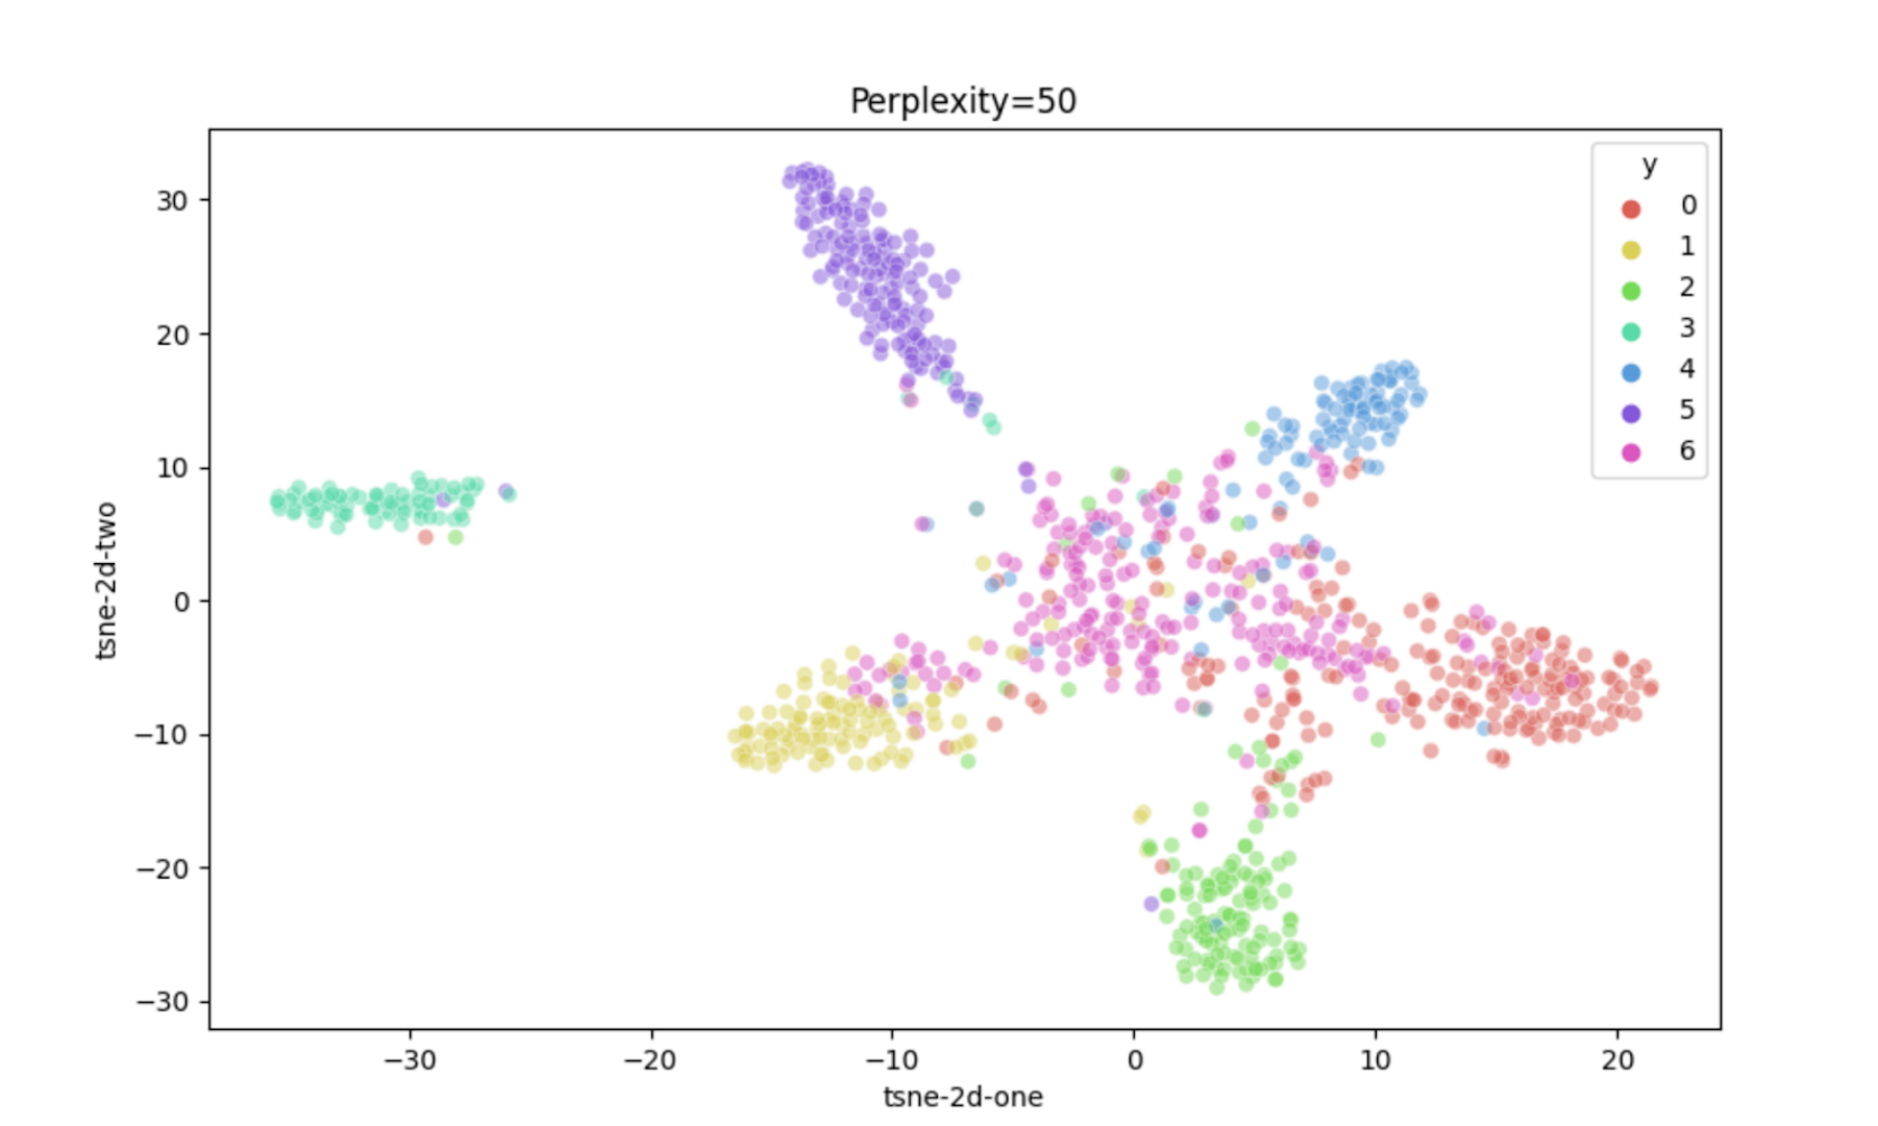}
       \caption{Feature space regularization}
       \label{fig:Ng2}
    \end{subfigure}
    \caption{Comparison of t-SNE plots for latent features of models using output space regularization versus feature space regularization. These plots are generated on the \textsc{PACS} dataset, with "Art Painting" as the test domain. Class 6 (pink) is the designated OOD class.}
\label{fig:reg-compare}
\end{figure*}

\subsection{Backbone-Agnostic Evaluation}

Our proposed framework is not dependent on any specific backbone and can be seamlessly integrated with any commonly used deep neural network. Empirically, we evaluated \sysname{}'s OOD detection performance against two of the best-performing baselines using two popular backbones in computer vision: VGG16 and WideResNet28-10. On the PACS dataset, the results are detailed in Table~\ref{tab:model_agnostic_auroc} and Table~\ref{tab:model_agnostic_aupr}. Clearly, \sysname{} consistently outperformed MBDG and MEDIC on both VGG16 and WideResNet28-10 backbones, demonstrating that its superior OOD detection capability is model-agnostic.

\begin{table*}[!t]
\centering
\setlength\tabcolsep{5pt}
\scriptsize
\caption{Performance comparison of using VGG16 and WRN28-10 backbone models for AUROC.}
\label{tab:model_agnostic_auroc}
\begin{tabular}{c|l|c|c|c|c|c}
\toprule
% \multirow{3}{*}{Network} & & \multicolumn{5}{c}{OOD Detection Algorithms} \\
% \cmidrule{3-7}
% & & \multicolumn{5}{c}{\textbf{AUROC}} \\
% \midrule
Network & Methods & MSP & Energy & DDU & OCSVM & Avg \\
\cmidrule{1-7}
\multirow{3}{*}{VGG16}
& MBDG  & 56.14 $\pm$ 4.07 & 60.10 $\pm$ 4.70 & 62.32 $\pm$ 7.91 & 41.68 $\pm$ 4.86 & 55.06 $\pm$ 2.56 \\
& MEDIC & NA & NA & NA & NA & 60.58 $\pm$ 3.10 \\
\cmidrule{2-7}
& \sysname{} (ours)  & 75.06 $\pm$ 1.21 & 78.56 $\pm$ 1.02 & 66.73 $\pm$ 2.31 & 47.92 $\pm$ 3.96 & 67.07 $\pm$ 1.56 \\
\cmidrule{1-7}
\multirow{3}{*}{WRN28-10}
& MBDG  & 62.38 $\pm$ 2.43 & 65.88 $\pm$ 3.82 & 56.06 $\pm$ 5.99 & 47.18 $\pm$ 5.06 & 57.88 $\pm$ 1.69 \\
& MEDIC & NA & NA & NA & NA & 59.07 $\pm$ 1.36 \\
\cmidrule{2-7}
& \sysname{} (ours)  & 67.97 $\pm$ 3.51 & 71.74 $\pm$ 3.97 & 57.48 $\pm$ 5.15 & 46.21 $\pm$ 1.71 & 60.85 $\pm$ 3.06 \\
\bottomrule
\end{tabular}
\end{table*}

\begin{table*}[!t]
\centering
\setlength\tabcolsep{5pt}
\scriptsize
\caption{Performance comparison of using VGG16 and WRN28-10 backbone models for AUPR.}
\label{tab:model_agnostic_aupr}
\begin{tabular}{c|l|c|c|c|c|c}
\toprule
% \multirow{3}{*}{Network} & & \multicolumn{5}{c}{OOD Detection Algorithms} \\
% \cmidrule{3-7}
% & & \multicolumn{5}{c}{\textbf{AUPR}} \\
% \midrule
Network & Methods & MSP & Energy & DDU & OCSVM & Avg \\
\cmidrule{1-7}
\multirow{3}{*}{VGG16}
& MBDG  & 16.49 $\pm$ 2.63 & 20.27 $\pm$ 3.43 & 24.72 $\pm$ 4.89 & 14.36 $\pm$ 1.78 & 18.96 $\pm$ 2.46 \\
& MEDIC & NA & NA & NA & NA & 21.94 $\pm$ 4.15 \\
\cmidrule{2-7}
& \sysname{} (ours)  & 26.72 $\pm$ 3.32 & 30.69 $\pm$ 2.00 & 22.19 $\pm$ 4.57 & 15.73 $\pm$ 4.31 & 23.83 $\pm$ 3.43 \\
\cmidrule{1-7}
\multirow{3}{*}{WRN28-10}
& MBDG  & 19.55 $\pm$ 2.95 & 22.51 $\pm$ 4.96 & 18.28 $\pm$ 4.69 & 13.62 $\pm$ 0.75 & 18.49 $\pm$ 3.23 \\
& MEDIC & NA & NA & NA & NA & 18.84 $\pm$ 2.59 \\
\cmidrule{2-7}
& \sysname{} (ours)  & 23.41 $\pm$ 5.15 & 26.66 $\pm$ 7.45 & 19.01 $\pm$ 4.70 & 13.31 $\pm$ 1.57 & 20.60 $\pm$ 4.62 \\
\bottomrule
\end{tabular}
\end{table*}

\subsection{Robustness Against Only Semantic Shift or Covariate Shift}

As shown in Table~\ref{tab:summary-all}, when only covariate shift exists (ID samples from an unknown target domain), our method achieved comparable or superior in-distribution classification accuracy compared to SOTA benchmarks, demonstrating its robustness against the covariate-shift-only setting (i.e., the conventional domain generalization setting). To evaluate its robustness against semantic shifts, we conducted additional experiments in which OODs were drawn from novel classes in the training domains. As shown in Table\ref{tab:semantic_shift_only}, our approach outperforms two of the best-performing baselines, MBDG and MEDIC, in detecting OOD under the semantic-shift-only setting, with improvements of up to 10\% in AUROC and 29\% in AUPR, demonstrating its robustness against semantic shifts.

\begin{table*}[!t]
\centering
\setlength\tabcolsep{5pt}
\scriptsize
\caption{OOD detection performance comparison with only semantic shift.}
\label{tab:semantic_shift_only}
\begin{tabular}{c|c|c}
\toprule
Method & \textbf{AUROC} & \textbf{AUPR} \\
\midrule
MBDG & 67.33 $\pm$ 2.78 & 28.17 $\pm$ 3.56 \\
MEDIC & 69.61 $\pm$ 4.30 & 28.98 $\pm$ 5.25 \\
Ours & 73.92 $\pm$ 2.37 & 36.29 $\pm$ 4.72 \\
\bottomrule
\end{tabular}
\end{table*}

\subsection{Complexity Analysis}

Regarding the time and space complexity, it is comparable to that of training a standard deep classifier.

The overall time complexity of the main training loop is $O(K \cdot (m \cdot T_{DNN} + n \cdot T_{DNN} + p))$, where:

\begin{itemize}
    \item $K$ represents the number of iterations in the outer loop until convergence.
    \item $m$ denotes the size of the minibatch.
    \item $n$ corresponds to the number of augmented OOD samples.
    \item $T_{DNN}$ is the time complexity of a forward pass, which depends on the specific network architecture design.
    \item $p$ IDicates the total number of parameters in the neural network.
\end{itemize}

The space complexity for the main training loop is $O(m + n + p)$.

\subsection{GDA Alone as OOD Detector}
While it is feasible to employ the fitted GDA as an OOD detector, our experiments show that GDA alone does not deliver satisfactory performance for OOD detection. Table~\ref{tab:gda_ood_detector} is a comparison of the AUROC and AUPR scores between a GDA OOD detector and our proposed method on the PACS dataset, it is obvious that our method significantly outperforms the GDA OOD detector.

\begin{table*}[!t]
\centering
\setlength\tabcolsep{5pt}
\scriptsize
\caption{Performance comparison of GDA OOD detector across different environments.}
\label{tab:gda_ood_detector}
\begin{tabular}{c|l|c|c|c|c|c}
\toprule
& Method & env 0 & env 1 & env 2 & env 3 & Avg \\
\midrule
\multirow{2}{*}{\textbf{AUROC}} 
& GDA & 53.47 $\pm$ 2.66 & 68.52 $\pm$ 7.77 & 55.47 $\pm$ 1.91 & 53.51 $\pm$ 3.04 & 57.74 $\pm$ 3.62 \\
& Ours & 75.29 $\pm$ 5.21 & 78.23 $\pm$ 4.85 & 84.15 $\pm$ 3.71 & 79.35 $\pm$ 5.11 & 79.25 $\pm$ 1.84 \\
\midrule
\multirow{2}{*}{\textbf{AUPR}} 
& GDA & 16.87 $\pm$ 3.28 & 25.54 $\pm$ 2.97 & 20.64 $\pm$ 3.06 & 14.78 $\pm$ 5.22 & 19.46 $\pm$ 2.36 \\
& Ours & 53.70 $\pm$ 1.17 & 53.43 $\pm$ 1.47 & 54.77 $\pm$ 1.55 & 53.74 $\pm$ 3.32 & 53.91 $\pm$ 0.29 \\
\bottomrule
\end{tabular}
\end{table*}

Although GDA struggles with accurately estimating input density outside the training support, it is fairly accurate for in-distribution samples drawn from the training set (see Table~\ref{tab:gda_training_set_id_performance}). Thus, GDA is sufficient to screen out "definitely not OOD" samples and accept the "likely OODs" to improve the separability between ID and OOD samples.

\begin{table*}[!t]
\centering
\setlength\tabcolsep{5pt}
\scriptsize
\caption{AUROC of GDA OOD Detector using the ID samples from the training set.}
\label{tab:gda_training_set_id_performance}
\begin{tabular}{c|c|c|c|c|c}
\toprule
Method & env 0 & env 1 & env 2 & env 3 & Avg \\
\midrule
GDA & 89.34 $\pm$ 1.55 & 92.83 $\pm$ 2.61 & 84.33 $\pm$ 0.91 & 86.72 $\pm$ 2.08 & 88.31 $\pm$ 8.70 \\
\bottomrule
\end{tabular}
\end{table*}
